# Supplementary material for: CoolerSpace: A Language for Physically Correct and Computationally Efficient Color Programming
Source: arXiv:2409.02771 source file (2024-09-04)
Supplement: Supplementary file 1 [file supplementary.pdf]

# CoolerSpace Supplementary Materials

## 1 CoolerSpace Language Specification

Sec. 1.1 defines the complete syntax of CoolerSpace. Sec. 1.2 defines permissible castings dictated by color science principles. Sec. 1.3 defines the formal typing rules.

### 1.1 CoolerSpace Syntax

Table 1: CoolerSpace syntax.

| | |
|---|---|
| Arrays | $a \in$ floating point arrays |
| Variable Names | $x \in$ variable names |
| Tristimulus Color Types | $\tau_{\text{tristimulus}} ::= \tau_{\text{XYZ}} \vert \tau_{\text{LMS}} \vert \tau_{\text{sRGB}} \vert \tau_{\text{opRGB}}$ |
| Perceptual Color Types | $\tau_{\text{perceptual}} ::= \tau_{\text{HSL}} \vert \tau_{\text{LAB}}$ |
| Color Types | $\tau_{\text{color}} ::= \tau_{\text{tristimulus}} \vert \tau_{\text{perceptual}}$ |
| Spectral Types | $\tau_{\text{spectrum}} ::= \tau_{\text{Light}} \vert \tau_{\text{Reflectance}} \vert \tau_{\text{Scattering}} \vert \tau_{\text{Absorption}} \vert \tau_{\text{Pigment}}$ |
| Physical Types | $\tau ::= \tau_{\text{color}} \vert \tau_{\text{spectrum}} \vert \tau_{\text{Chromaticity}} \vert \tau_{\text{Matrix}}$ |
| Dimension Types | $d ::= \mathbb{N} \vert d \times d$ |
| Shaped Types | $s ::= (\tau, d)$ |
| XYZ Channels | $c_{\text{XYZ}} ::= X \vert Y \vert Z$ |
| LMS Channels | $c_{\text{LMS}} ::= L \vert M \vert S$ |
| sRGB Channels | $c_{\text{sRGB}} ::= R \vert G \vert B$ |
| opRGB Channels | $c_{\text{opRGB}} ::= R \vert G \vert B$ |
| HSV Channels | $c_{\text{HSL}} ::= H \vert S \vert V$ |
| LAB Channels | $c_{\text{LAB}} ::= L \vert A \vert B$ |
| Channels | $c ::= c_{\text{XYZ}} \vert c_{\text{LMS}} \vert c_{\text{sRGB}} \vert c_{\text{opRGB}} \vert c_{\text{HSL}} \vert c_{\text{LAB}}$ |
| Binary Operators | $\oplus ::= + \vert - \vert \times \vert /$ |
| Values | $v ::= x \vert \tau(a) \vert \tau(v) \vert \tau(v, v) \vert \mathsf{mix}(v, v, v, v) \vert v \oplus v \vert \mathsf{matmul}(v, v) \vert v.c$ |
| Expressions | $e ::= x = v$ |
| Programs | $P ::= e; P \vert e$ |

### 1.2 Casting Graph

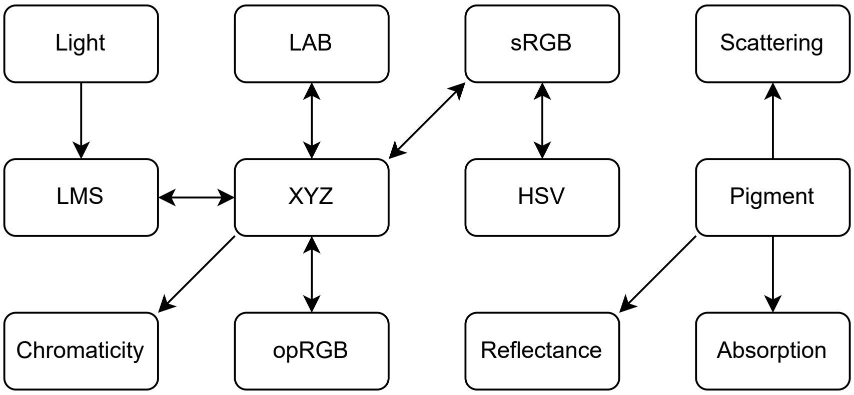


Figure 1: The graph showing all permissible castings.

### 1.3 CoolerSpace Type System

$$\frac{\tau \notin \{\tau_{\text{Pigment}}, \tau_{\text{Matrix}}\} \qquad d_1 = d_2 \times \mathsf{channel\_count}(t) \qquad a : d_1}{\Gamma \vdash \tau(a) : (t, d_2)} \textsc{Init}$$

$$\frac{a : d}{\Gamma \vdash \tau_{\text{Matrix}}(a) : (\tau_{\text{Matrix}}, d)} \textsc{MatrixInit}$$

$$\frac{\Gamma \vdash v_1 : (\tau_{\text{Absorption}}, d) \qquad \Gamma \vdash v_2 : (\tau_{\text{Scattering}}, d)}{\Gamma \vdash \tau_{\text{Pigment}}(v_1, v_2) : (\tau_{\text{Pigment}}, d)} \textsc{PigmentInit}$$

$$\frac{}{\mathsf{broadcastable}(d, d)} \textsc{TrivialBroadcast}$$

$$\frac{}{\mathsf{broadcastable}(1, d)} \textsc{ScalarBroadcast}$$

$$\frac{d_1 = d_2 \times d_3}{\mathsf{broadcastable}(d_3, d_1)} \textsc{SubsetBroadcast}$$

$$\frac{\Gamma \vdash v_1 : (\tau_{\text{Light}}, d) \qquad \Gamma \vdash v_2 : (\tau_{\text{Light}}, d)}{\Gamma \vdash v_1 + v_2 : (\tau_{\text{Light}}, d)} \textsc{LightAdd}$$

$$\frac{\Gamma \vdash v_1 : (\tau_{\text{tristimulus}}, d) \qquad \Gamma \vdash v_2 : (\tau_{\text{tristimulus}}, d)}{\Gamma \vdash v_1 + v_2 : (\tau_{\text{tristimulus}}, d)} \textsc{TristimulusAdd}$$

$$\frac{\Gamma \vdash v_1 : (\tau_{\text{perceptual}}, d) \qquad \Gamma \vdash v_2 : (\tau_{\text{perceptual}}, d)}{\Gamma \vdash v_1 + v_2 : (\tau_{\text{perceptual}}, d)} \textsc{PerceptualAdd}$$

$$\frac{\Gamma \vdash v_1 : (\tau_{\text{Matrix}}, d_1) \qquad \Gamma \vdash v_2 : (\tau_{\text{Matrix}}, d_2) \qquad \mathsf{broadcastable}(d_2, d_1)}{\Gamma \vdash v_1 + v_2 : (\tau_{\text{Matrix}}, d_1)} \textsc{MatrixAddL}$$

$$\frac{\Gamma \vdash v_1 : (\tau_{\text{Matrix}}, d_1) \qquad \Gamma \vdash v_2 : (\tau_{\text{Matrix}}, d_2) \qquad \mathsf{broadcastable}(d_1, d_2)}{\Gamma \vdash v_1 + v_2 : (\tau_{\text{Matrix}}, d_2)} \textsc{MatrixAddR}$$

$$\frac{\Gamma \vdash v_1 : (\tau_{\text{Light}}, d) \qquad \Gamma \vdash v_2 : (\tau_{\text{Reflectance}}, d)}{\Gamma \vdash v_1 \times v_2 : (\tau_{\text{Light}}, d)} \textsc{Reflect}$$

$$\frac{\Gamma \vdash v_1 : (\tau_{\text{tristimulus}}, d) \qquad \Gamma \vdash v_2 : (\tau_{\text{Matrix}}, \mathsf{channel\_count}(\tau_{\text{tristimulus}}))}{\Gamma \vdash v_1 \times v_2 : (\tau_{\text{tristimulus}}, d)} \textsc{TriChScale}$$

$$\frac{\Gamma \vdash v_1 : (\tau_{\text{Matrix}}, d_1) \qquad \Gamma \vdash v_2 : (\tau_{\text{Matrix}}, d_2) \qquad \mathsf{broadcastable}(d_2, d_1)}{\Gamma \vdash v_1 \times v_2 : (\tau_{\text{Matrix}}, d_1)} \textsc{MatrixMulL}$$

$$\frac{\Gamma \vdash v_1 : (\tau_{\text{Matrix}}, d_1) \qquad \Gamma \vdash v_2 : (\tau_{\text{Matrix}}, d_2) \qquad \mathsf{broadcastable}(d_1, d_2)}{\Gamma \vdash v_1 \times v_2 : (\tau_{\text{Matrix}}, d_2)} \textsc{MatrixMulR}$$

$$\frac{\Gamma \vdash v_1 : (\tau_{\text{Matrix}}, d_1) \qquad \Gamma \vdash v_2 : (\tau_{\text{Matrix}}, d_2) \qquad \mathsf{broadcastable}(d_2, d_1)}{\Gamma \vdash v_1 / v_2 : (\tau_{\text{Matrix}}, d_1)} \textsc{MatrixDivL}$$

$$\frac{\Gamma \vdash v_1 : (\tau_{\text{Matrix}}, d_1) \qquad \Gamma \vdash v_2 : (\tau_{\text{Matrix}}, d_2) \qquad \mathsf{broadcastable}(d_1, d_2)}{\Gamma \vdash v_1 / v_2 : (\tau_{\text{Matrix}}, d_2)} \textsc{MatrixDivR}$$

$$\frac{\Gamma \vdash v_1 : (\tau_{\text{tristimulus}}, d) \qquad \Gamma \vdash v_2 : (\tau_{\text{Matrix}}, \mathsf{channel\_count}(\tau_{\text{tristimulus}}) \times \mathsf{channel\_count}(\tau_{\text{tristimulus}}))}{\Gamma \vdash \mathsf{matmul}(v_1, v_2) : (\tau_{\text{tristimulus}}, d)} \textsc{TriMatMul}$$

$$\frac{\Gamma \vdash v_1 : (\tau_{\text{Matrix}}, d_1 \times \mathbb{N}) \qquad \Gamma \vdash v_2 : (\tau_{\text{Matrix}}, \mathbb{N} \times d_2)}{\Gamma \vdash \mathsf{matmul}(v_1, v_2) : (\tau_{\text{Matrix}}, d_1 \times d_2)} \textsc{MatMul}$$

$$\frac{\Gamma \vdash v_1, v_2 : (\tau_{\text{Pigment}}, d) \qquad \Gamma \vdash v_3, v_4 : (\tau_{\text{Matrix}}, d)}{\Gamma \vdash \mathsf{mix}(v_3, v_1, v_4, v_2) : (\tau_{\text{Pigment}}, d)} \textsc{PigmentMix}$$

$$\frac{\Gamma \vdash v : (\tau_1, d) \qquad \mathsf{path\_exists}(\tau_1, \tau_2)}{\Gamma \vdash \tau_2(v) : (\tau_2, d)} \textsc{Cast}$$

$$\frac{\tau \neq \tau_{\text{Pigment}} \qquad \Gamma \vdash v : (\tau, d)}{\Gamma \vdash \tau_{\text{Matrix}}(v) : (\tau_{\text{Matrix}}, d \times \mathsf{channel\_count}(\tau))} \textsc{MatrixCast}$$

$$\frac{\Gamma \vdash v : (\tau_i, d) \qquad c \in c_i}{\Gamma \vdash v.c : (\tau_{\text{Matrix}}, d)} \textsc{ChannelGet}$$

Figure 2: CoolerSpace typing rules. $\mathsf{path\_exists}(\tau_1, \tau_2)$ in the Cast rule type checks only if there exists a path from $\tau_1$ to $\tau_2$ in Fig. 1.

# 2 Translational Soundness

Programs written in CoolerSpace are translated to ONNX [11]. This section proves that CoolerSpace is translationally sound. For the translation between CoolerSpace to ONNX to be sound, every well-typed value in CoolerSpace must be translated to a well-typed value in ONNX. Translational soundness indicates that our translation preserves typeability: the type safety of CoolerSpace is as strong as that of ONNX.

To succinctly demonstrate our proof strategy without losing generality, we have defined a subset of our language, dubbed SmallerSpace (Sec. 2.1). The syntax for SmallerSpace can be found in Tbl. 3, and the corresponding type rules can be found in Fig. 3. We have also formalized a subset of ONNX that is relevant to our translation (Sec. 2.2). The syntax can be found in Tbl. 4, and the corresponding type rules are in Fig. 4. Sec. 2.3 defines the formal translational semantics from SmallerSpace to ONNX. Sec. 2.4 shows the proof of translational soundness.

Tbl. 2 defines a channel count lookup table that will be referenced by the $\mathsf{channel\_count}(\cdot)$ function used during translation and type checking in this section.

$$\begin{aligned}
&\mathsf{channel_count}(\tau_{\text{LMS}}) = 3\\
&\mathsf{channel_count}(\tau_{\text{XYZ}}) = 3\\
&\mathsf{channel_count}(\tau_{\text{Light}}) = 89\\
&\mathsf{channel_count}(\tau_{\text{Reflectance}}) = 89
\end{aligned}$$

Table 2: Channel count lookup table

## 2.1 SmallerSpace Syntax and Typing Rules

| | |
|---|---|
| Natural numbers | $\mathbb{N} \in$ natural numbers |
| Arrays | $a \in$ floating point array literals |
| Dimension types | $d ::= \mathbb{N} \| d \times d$ |
| Color types | $\tau_{\text{color}} ::= \tau_{\text{XYZ}} \| \tau_{\text{LMS}} \| \tau_{\text{sRGB}}$ |
| Spectral types | $\tau_{\text{spectrum}} ::= \tau_{\text{Light}} \| \tau_{\text{Reflectance}}$ |
| Physical types | $\tau ::= \tau_{\text{color}} \| \tau_{\text{spectrum}}$ |
| Shaped types | $s ::= (\tau, d)$ |
| Values | $v ::= \tau(a) \| \tau(v) \| v + v \| v \times v$ |

Table 3: SmallerSpace syntax

$$\frac{d_1 = d_2 \times \mathsf{channel\_count}(\tau) \qquad a : d_1}{\tau(a) : (\tau, d_2)}\ \textsc{Init}$$

$$\frac{v : (\tau_1, d) \qquad \mathsf{path\_exists}(\tau_1, \tau_2)}{\tau_2(v) : (\tau_2, d)}\ \textsc{Cast}$$

$$\frac{v_1, v_2 : (\tau_{\text{color}}, d)}{v_1 + v_2 : (\tau_{\text{color}}, d)}\ \textsc{ColorAdd}$$

$$\frac{v_1, v_2 : (\tau_{\text{Light}}, d)}{v_1 + v_2 : (\tau_{\text{Light}}, d)}\ \textsc{LightAdd}$$

$$\frac{v_1 : (\tau_{\text{Light}}, d) \qquad v_2 : (\tau_{\text{Reflectance}}, d)}{v_1 \times v_2 : (\tau_{\text{Light}}, d)}\ \textsc{Reflect}$$

Figure 3: SmallerSpace type rules.

## 2.2 ONNX Syntax and Typing Rules

| | |
|---|---|
| Natural Numbers | $\mathbb{N} \in$ natural numbers |
| Arrays | $a \in$ floating point arrays |
| Dimension Types | $d ::= \mathbb{N} \mid d \times d$ |
| Values | $u ::= a \mid \mathsf{add}(u,u) \mid \mathsf{div}(u,u) \mid \mathsf{mul}(u,u)$ <br> $\mid \mathsf{sub}(u,u) \mid \mathsf{matmul}(u,u) \mid \mathsf{pow}(u,u)$ |

Table 4: Simplified ONNX syntax.

$$\frac{}{\mathsf{broadcastable}(d, d)}\ \textsc{TrivialBroadcast}$$

$$\frac{}{\mathsf{broadcastable}(1, d)}\ \textsc{ScalarBroadcast}$$

$$\frac{d_1 = d_2 \times d_3}{\mathsf{broadcastable}(d_3, d_1)}\ \textsc{SubsetBroadcast}$$

$$\frac{u_1 : d_1 \qquad u_2 : d_2 \qquad \mathsf{broadcastable}(d_2, d_1)}{\mathsf{add}(u_1, u_2) : d_1}\ \textsc{OnnxAddL}$$

$$\frac{u_1 : d_1 \qquad u_2 : d_2 \qquad \mathsf{broadcastable}(d_1, d_2)}{\mathsf{add}(u_1, u_2) : d_2}\ \textsc{OnnxAddR}$$

$$\frac{u_1 : d_1 \qquad u_2 : d_2 \qquad \mathsf{broadcastable}(d_2, d_1)}{\mathsf{sub}(u_1, u_2) : d_1}\ \textsc{OnnxSubL}$$

$$\frac{u_1 : d_1 \qquad u_2 : d_2 \qquad \mathsf{broadcastable}(d_1, d_2)}{\mathsf{sub}(u_1, u_2) : d_2}\ \textsc{OnnxSubR}$$

$$\frac{u_1 : d_1 \qquad u_2 : d_2 \qquad \mathsf{broadcastable}(d_2, d_1)}{\mathsf{mul}(u_1, u_2) : d_1}\ \textsc{OnnxMulL}$$

$$\frac{u_1 : d_1 \qquad u_2 : d_2 \qquad \mathsf{broadcastable}(d_1, d_2)}{\mathsf{mul}(u_1, u_2) : d_2}\ \textsc{OnnxMulR}$$

$$\frac{u_1 : d_1 \qquad u_2 : d_2 \qquad \mathsf{broadcastable}(d_2, d_1)}{\mathsf{div}(u_1, u_2) : d_1}\ \textsc{OnnxDivL}$$

$$\frac{u_1 : d_1 \qquad u_2 : d_2 \qquad \mathsf{broadcastable}(d_1, d_2)}{\mathsf{div}(u_1, u_2) : d_2}\ \textsc{OnnxDivR}$$

$$\frac{u_1 : d_1 \qquad u_2 : d_2 \qquad \mathsf{broadcastable}(d_2, d_1)}{\mathsf{pow}(u_1, u_2) : d_1}\ \textsc{OnnxPowL}$$

$$\frac{u_1 : d_1 \qquad u_2 : d_2 \qquad \mathsf{broadcastable}(d_1, d_2)}{\mathsf{pow}(u_1, u_2) : d_2}\ \textsc{OnnxPowR}$$

Figure 4: Simplified ONNX type rules.

## 2.3 Translational Semantics

| | |
|---|---|
| $[\![\mathbb{N}]\!] \triangleq \mathbb{N}$ | **T-Nat** |
| $[\![v_1 + v_2]\!] \triangleq \Phi(+, \tau_1, \tau_2)(v_1, v_2), \quad v_1 : (\tau_1, d_1),\ v_2 : (\tau_2, d_2)$ | **T-Add** |
| $[\![a]\!] \triangleq a$ | **T-Array** |
| $[\![v_1 \times v_2]\!] \triangleq \Phi(\times, \tau_1, \tau_2)(v_1, v_2), \quad v_1 : (\tau_1, d_1),\ v_2 : (\tau_2, d_2)$ | **T-Mul** |
| $[\![\tau(a)]\!] \triangleq a$ | **T-Init** |
| $[\![\tau_d(v_o)]\!] \triangleq \Psi(\tau_o, \tau_d)(v_o), \quad v_o : (\tau_o, d_o)$ | **T-Cast** |
| $[\![d]\!] \triangleq d$ | **T-Dim** |
| $[\![(\tau, d)]\!] \triangleq d \times \mathsf{channel\_count}(\tau)$ | **T-Type** |
| $\Phi(+, \tau_{\text{XYZ}}, \tau_{\text{XYZ}})(v_1, v_2) \triangleq \mathsf{add}\,([\![v_1]\!], [\![v_2]\!])$ | |
| $\Phi(+, \tau_{\text{LMS}}, \tau_{\text{LMS}})(v_1, v_2) \triangleq \mathsf{add}\,([\![v_1]\!], [\![v_2]\!])$ | |
| $\Phi(+, \tau_{\text{sRGB}}, \tau_{\text{sRGB}})(v_1, v_2) \triangleq \mathsf{mul}(\mathsf{pow}(\mathsf{add}(\mathsf{pow}(\mathsf{div}([\![v_1]\!], [255]), [2.2]), \mathsf{div}(\mathsf{pow}([\![v_2]\!], [255])\ [2.2])), [0.455]), [255])$ | |
| $\Phi(\times, \tau_{\text{Light}}, \tau_{\text{Reflectance}})(v_1, v_2) \triangleq \mathsf{mul}([\![v_1]\!], [\![v_2]\!])$ | |
| $\Psi(\tau_{\text{Light}}, \tau_{\text{LMS}})(v) \triangleq \mathsf{matmul}\,([\![v]\!], \mathrm{M}_1)$ | |
| $\Psi(\tau_{\text{LMS}}, \tau_{\text{XYZ}})(v) \triangleq \mathsf{matmul}\,([\![v]\!], \mathrm{M}_2)$ | |
| $\Psi(\tau_{\text{XYZ}}, \tau_{\text{sRGB}})(v) \triangleq \mathsf{pow}\left(\mathsf{mul}\left(\mathsf{matmul}\left([\![v]\!], \mathrm{M}_3\right), [255]\right), [2.2]\right)$ | |

Table 5: SmallerSpace to ONNX translational semantics. $\mathrm{M}_1$, $\mathrm{M}_2$, and $\mathrm{M}_3$ represent the LMS Cone Fundamentals, XYZ to LMS transformation matrix, and XYZ to RGB transformation matrix, respectively. They are constant matrices that can be found in standard color science texts [15], and are omitted here.

## 2.4 Translational Soundness Proof

**Theorem.** The theorem for translational soundness is given below:

$$\frac{\llbracket v : (\tau, d) \rrbracket}{\llbracket v \rrbracket : \llbracket (\tau, d) \rrbracket}$$

We will prove the theorem through structural induction. The induction hypothesis can be generally stated as follows:

$$\frac{\llbracket v_i \subset v \rrbracket \qquad \llbracket v_i : (\tau_i, d_i) \rrbracket \qquad \llbracket v : (\tau, d) \rrbracket}{\llbracket v_i \rrbracket : \llbracket (\tau_i, d_i) \rrbracket}\ \textsc{IndHyp}$$

We will be using the converse of several typing rules in SMALLERSPACE. These rules will be labeled as CONV-RULENAME. In order for a converse rule to be valid, the set of expressions that are type checked by a rule must only be type check-able by said rule. We will show this assumption to be true for every case. We also use the SUBST rule to indicate substitution of equivalent values.

In this proof we iterate over every rule in SMALLERSPACE, and show that each rule is translationally sound.

### Base case: Init

Values of the form $\tau(a)$ do not have value subterms. This makes it our base case for induction. There is only one type rule under which $\tau(a)$ type checks: INIT. Therefore CONV-INIT is valid. We also introduce a new rule T-ARRTYPE to assist with this proof. T-ARRTYPE ensures that the dimension type of an array literal is preserved after translation.

$$\frac{\llbracket a : d \rrbracket}{\llbracket a \rrbracket : \llbracket d \rrbracket}\ \text{T-}\textsc{ArrType}$$

Given $\llbracket \tau(a) : (\tau, d) \rrbracket$, we can conclude that the translated type of $\llbracket \tau(a) \rrbracket$ is $d \times \mathsf{channel\_count}(\tau)$.

$$\dfrac{\dfrac{\dfrac{\dfrac{\dfrac{\llbracket \tau(a) : (\tau, d) \rrbracket}{\llbracket a : d \times \mathsf{channel\_count}(\tau) \rrbracket}\ \textsc{Conv-Init}}{\llbracket a \rrbracket : \llbracket d \times \mathsf{channel\_count}(\tau) \rrbracket}\ \text{T-}\textsc{ArrType} \qquad \dfrac{}{\llbracket a \rrbracket \triangleq a}\ \text{T-}\textsc{Array}}{a : \llbracket d \times \mathsf{channel\_count}(\tau) \rrbracket}\ \textsc{Subst} \qquad \dfrac{}{\llbracket \tau(a) \rrbracket \triangleq a}\ \text{T-}\textsc{Init}}{\llbracket \tau(a) \rrbracket : \llbracket d \times \mathsf{channel\_count}(\tau) \rrbracket} \qquad \dfrac{}{\llbracket d \times \mathsf{channel\_count}(\tau) \rrbracket \triangleq d \times \mathsf{channel\_count}(\tau)}\ \text{T-}\textsc{Dim}}{\llbracket \tau(a) \rrbracket : d \times \mathsf{channel\_count}(\tau)}\ \textsc{Subst}$$

$\llbracket (\tau, d) \rrbracket$ also translates to $d \times \mathsf{channel\_count}(\tau)$. Therefore, we can conclude that $\llbracket \tau(a) \rrbracket : \llbracket (\tau, d) \rrbracket$. This satisfies the translational soundness theorem.

$$\dfrac{\llbracket \tau(a) \rrbracket : d \times \mathsf{channel\_count}(\tau) \qquad \dfrac{}{\llbracket (\tau, d) \rrbracket \triangleq d \times \mathsf{channel\_count}(\tau)}\ \text{T-}\textsc{Type}}{\llbracket \tau(a) \rrbracket : \llbracket (\tau, d) \rrbracket}\ \textsc{Subst}$$

### Case 1: ColorAdd

In order for Conv-ColorAdd to be a valid rule, the set of expressions that are type checked by ColorAdd must only be type check-able by ColorAdd. In other words, $v_1 + v_2 : (\tau_{\text{color}}, d)$ must type check if and only if the premises for ColorAdd are satisfied. We know this to be true, as there is no other rule that type checks addition between color types.

The proof below shows the validity of ColorAdd for $\tau_{\text{XYZ}} + \tau_{\text{XYZ}}$. This proof must be repeated for LMS and sRGB.

$$\dfrac{\dfrac{\dfrac{\dfrac{\llbracket v_1 + v_2 : (\tau_{\text{XYZ}}, d)\rrbracket}{\llbracket v_1, v_2 : (\tau_{\text{XYZ}}, d)\rrbracket}\ \textsc{Conv-ColorAdd} \qquad \llbracket v_1, v_2 \subset v_1 + v_2\rrbracket}{\llbracket v_1, v_2\rrbracket : \llbracket(\tau_{\text{XYZ}}, d)\rrbracket}\ \textsc{IndHyp} \qquad \dfrac{}{\mathsf{broadcastable}(\llbracket(\tau_{\text{XYZ}}, d)\rrbracket, \llbracket(\tau_{\text{XYZ}}, d)\rrbracket)}\ \textsc{TrivBroad}}{\mathsf{add}(\llbracket v_1\rrbracket, \llbracket v_2\rrbracket) : \llbracket(\tau_{\text{XYZ}}, d)\rrbracket}\ \textsc{OnnxAddR} \qquad \dfrac{\llbracket v_1, v_2 : (\tau_{\text{XYZ}}, d)\rrbracket}{\llbracket v_1 + v_2\rrbracket \triangleq \mathsf{add}(\llbracket v_1\rrbracket, \llbracket v_2\rrbracket)}\ \textsc{T-Add}}{\llbracket v_1 + v_2\rrbracket : \llbracket(\tau_{\text{XYZ}}, d)\rrbracket}\ \textsc{Subst}$$

### Case 2: LightAdd

Like ColorAdd, LightAdd is the only rule that can type check $v_1 + v_2 : (\tau_{\text{Light}}, d)$. Thus, Conv-LightAdd is valid. The proof tree is similar to that of ColorAdd.

$$\dfrac{\dfrac{\dfrac{\dfrac{\llbracket v_1 + v_2 : (\tau_{\text{Light}}, d)\rrbracket}{\llbracket v_1, v_2 : (\tau_{\text{Light}}, d)\rrbracket}\ \textsc{Conv-LightAdd} \qquad \llbracket v_1, v_2 \subset v_1 + v_2\rrbracket}{\llbracket v_1, v_2\rrbracket : \llbracket(\tau_{\text{Light}}, d)\rrbracket}\ \textsc{IndHyp} \qquad \dfrac{}{\mathsf{broadcastable}(\llbracket(\tau_{\text{Light}}, d)\rrbracket, \llbracket(\tau_{\text{Light}}, d)\rrbracket)}\ \textsc{TrivBroad}}{\mathsf{add}(\llbracket v_1\rrbracket, \llbracket v_2\rrbracket) : \llbracket(\tau_{\text{Light}}, d)\rrbracket}\ \textsc{OnnxAddR} \qquad \dfrac{\llbracket v_1, v_2 : (\tau_{\text{Light}}, d)\rrbracket}{\llbracket v_1 + v_2\rrbracket \triangleq \mathsf{add}(\llbracket v_1\rrbracket, \llbracket v_2\rrbracket)}\ \textsc{T-Add}}{\llbracket v_1 + v_2\rrbracket : \llbracket(\tau_{\text{Light}}, d)\rrbracket}\ \textsc{Subst}$$

### Case 3: Reflect

Reflect is the only way by which $v_1 \times v_2$ is type checked in SmallerSpace. Therefore Conv-Reflect is valid. Given $\llbracket v_1 \times v_2 : (\tau_{\text{Light}}, d)\rrbracket$, we can conclude that $\llbracket v_1\rrbracket$ and $\llbracket v_2\rrbracket$ are of type $d \times \mathsf{channel\_count}(\tau_{\text{Light}})$ after translation.

$$\dfrac{\dfrac{\dfrac{\llbracket v_1 \times v_2 : (\tau_{\text{Light}}, d)\rrbracket}{\llbracket v_1 : (\tau_{\text{Light}}, d)\rrbracket}\ \textsc{Conv-Reflect} \qquad \llbracket v_1 \subset v_1 \times v_2\rrbracket}{\llbracket v_1\rrbracket : \llbracket(\tau_{\text{Light}}, d)\rrbracket}\ \textsc{IndHyp}}{\llbracket v_1\rrbracket : d \times \mathsf{channel\_count}(\tau_{\text{Light}})}\ \textsc{T-Dim}$$

$$\dfrac{\dfrac{\dfrac{\dfrac{\llbracket v_1 \times v_2 : (\tau_{\text{Light}}, d)\rrbracket}{\llbracket v_2 : (\tau_{\text{Reflectance}}, d)\rrbracket}\ \textsc{Inv-Reflect} \qquad \llbracket v_2 \subset v_1 \times v_2\rrbracket}{\llbracket v_2\rrbracket : \llbracket(\tau_{\text{Reflectance}}, d)\rrbracket}\ \textsc{IndHyp}}{\llbracket v_2\rrbracket : d \times \mathsf{channel\_count}(\tau_{\text{Reflectance}})}\ \textsc{T-Dim} \qquad \mathsf{channel\_count}(\tau_{\text{Reflectance}}) = \mathsf{channel\_count}(\tau_{\text{Light}})}{\llbracket v_2\rrbracket : d \times \mathsf{channel\_count}(\tau_{\text{Light}})}\ \textsc{Subst}$$

With this information, we can show that $\mathsf{mul}([\![v_1]\!], [\![v_2]\!]) : d \times \mathsf{channel\_count}(\tau_{\text{Light}})$.

$$\dfrac{[\![v_1]\!] : d \times \mathsf{channel\_count}(\tau_{\text{Light}}) \qquad [\![v_2]\!] : d \times \mathsf{channel\_count}(\tau_{\text{Light}}) \qquad \dfrac{}{\mathsf{broadcastable}(d \times \mathsf{channel\_count}(\tau_{\text{Light}}), d \times \mathsf{channel\_count}(\tau_{\text{Light}}))}\,\textsc{TrivBroad}}{\mathsf{mul}([\![v_1]\!], [\![v_2]\!]) : d \times \mathsf{channel\_count}(\tau_{\text{Light}})}\,\textsc{OnnxMulR}$$

Since $v_1 \times v_2$ is translated to $\mathsf{mul}([\![v_1]\!], [\![v_2]\!])$ with type $d \times \mathsf{channel\_count}(\tau_{\text{Light}})$, and since $[\![(\tau_{\text{Light}}, d)]\!]$ is also typed $d \times \mathsf{channel\_count}(\tau_{\text{Light}})$ after translation, we can conclude that Reflect is translationally sound.

$$\dfrac{\dfrac{\mathsf{mul}([\![v_1]\!], [\![v_2]\!]) : d \times \mathsf{channel\_count}(\tau_{\text{Light}}) \qquad \dfrac{[\![v_1 : (\tau_{\text{Light}}, d)]\!] \quad [\![v_2 : (\tau_{\text{Reflectance}}, d)]\!]}{[\![v_1 \times v_2]\!] \triangleq \mathsf{mul}([\![v_1]\!], [\![v_2]\!])}\,\text{T-Mul}}{[\![v_1 \times v_2]\!] : d \times \mathsf{channel\_count}(\tau_{\text{Light}})}\,\textsc{Subst} \qquad \dfrac{}{[\![(\tau_{\text{Light}}, d)]\!] \triangleq d \times \mathsf{channel\_count}(\tau_{\text{Light}})}\,\text{T-}\textsc{Type}}{[\![v_1 \times v_2]\!] : [\![(\tau_{\text{Light}}, d)]\!]}\,\textsc{Subst}$$

**Case 4: Cast**

For any output physical type, there are multiple origin physical types that can satisfy the Cast rule. Therefore, we must show that Cast is translationally sound for every pair of types $\tau_1, tau_2$ such that $\mathsf{path\_exists}(\tau_1, \tau_2)$. All these proofs are similar in structure. I will be showing the proof for `Light` to `LMS`.



We first show that $[\![v]\!]$ is of type $d \times \mathsf{channel\_count}(\tau_{\text{Light}})$ after translation.

$$\dfrac{\dfrac{\dfrac{[\![\tau_{\text{LMS}}(v) : (\tau_{\text{LMS}}, d)]\!]}{[\![v : (\tau_{\text{Light}}, d)]\!]}\,\textsc{Conv-Cast-Light2LMS} \qquad [\![v \subset \tau_{\text{LMS}}(v)]\!]}{[\![v]\!] : [\![(\tau_{\text{Light}}, d)]\!]}\,\textsc{IndHyp} \qquad \dfrac{}{[\![(\tau_{\text{Light}}, d)]\!] \triangleq d \times \mathsf{channel\_count}(\tau_{\text{Light}})}\,\text{T-}\textsc{Type}}{[\![v]\!] : d \times \mathsf{channel\_count}(\tau_{\text{Light}})}\,\textsc{Subst}$$

$[\![\tau_{\text{LMS}}(v)]\!]$ translates to $\mathsf{matmul}([\![v]\!], M_1)$, where $M_1$ is a constant matrix of dimension $\mathsf{channel\_count}(\tau_{\text{Light}}) \times \mathsf{channel\_count}(\tau_{\text{LMS}})$.

$$\dfrac{[\![v : (\tau_{\text{Light}}, d)]\!]}{[\![\tau_{\text{LMS}}(v)]\!] \triangleq \mathsf{matmul}([\![v]\!], M_1)}\,\text{T-}\textsc{Cast}$$

We can conclude that $[\![\tau_{\text{LMS}}(v)]\!] : d \times \mathsf{channel\_count}(\tau_{\text{LMS}})$.

$$\dfrac{\dfrac{[\![v]\!] : d \times \mathsf{channel\_count}(\tau_{\text{Light}}) \qquad M_1 : \mathsf{channel\_count}(\tau_{\text{Light}}) \times \mathsf{channel\_count}(\tau_{\text{LMS}})}{\mathsf{matmul}([\![v]\!], M_1) : d \times \mathsf{channel\_count}(\tau_{\text{LMS}})}\,\textsc{OnnxMatMul} \qquad [\![\tau_{\text{LMS}}(v)]\!] \triangleq \mathsf{matmul}([\![v]\!], M_1)}{[\![\tau_{\text{LMS}}(v)]\!] : d \times \mathsf{channel\_count}(\tau_{\text{LMS}})}\,\textsc{Subst}$$

Since $[\![(\tau_{\text{LMS}}, d)]\!]$ also translates to $d \times \mathsf{channel\_count}(\tau_{\text{LMS}})$, the translational soundness theorem holds true for the Cast rule when the origin type is $\tau_{\text{Light}}$ and the destination type is $\tau_{\text{LMS}}$.

$$\dfrac{[\![\tau_{\text{LMS}}(v)]\!] : d \times \mathsf{channel\_count}(\tau_{\text{LMS}}) \qquad \dfrac{}{[\![(\tau_{\text{LMS}}, d)]\!] \triangleq d \times \mathsf{channel\_count}(\tau_{\text{LMS}})}\ \text{T-Type}}{[\![\tau_{\text{LMS}}(v)]\!] : [\![(\tau_{\text{LMS}}, d)]\!]}\ \text{Subst}$$

Translational soundness for Cast must be proven for every valid pair of origin and destination types. The remaining Cast proofs are of similar form to the one above.

### Conclusion

We have shown that every rule in SmallerSpace is translationally sound under the inductive hypothesis. We have also proven that a base case, Init, is translationally sound independent of the inductive hypothesis. Therefore, by the principle of structural induction, SmallerSpace must be translationally sound.

# 3 Type Soundness Background Information

We can additionally show that CoolerSpace is type sound. In this section we will describe the requisite information for the type soundness proof. Similar to our proof of translational soundness, We will prove type soundness over SmallerSpace, a subset of CoolerSpace. We define SmallerSpace's syntax and type rules in Sec. 3.1. Evaluation rules are specified in Sec. 3.2. These evaluation rules represent the expected computation for each operation. In Sec. 4, we will utilize the information outlined in this section to prove that SmallerSpace is type sound.

### 3.1 SmallerSpace Syntax and Rules

The SmallerSpace syntax that we use here has been augmented with array expressions. These array expressions allow us to perform arithmetic on raw floating point arrays, akin to NumPy array operations. Like ONNX, broadcasting rules are also used in array expressions. The syntax for SmallerSpace can be found in Tbl. 6, and the corresponding type rules can be found in Fig. 5.

| | |
|---|---|
| Natural numbers | $\mathbb{N} \in$ natural numbers |
| Binary operators | $\oplus ::= + \mid - \mid \times \mid / \mid **$ |
| Arrays | $a \in \mathbb{A}$ (set of floating point array literals) |
| Array Expressions | $\alpha ::= a \mid (\alpha) \oplus (\alpha) \mid \mathsf{matmul}(\alpha, \alpha)$ |
| Dimension types | $d ::= \mathbb{N} \mid d \times d$ |
| Tristimulus types | $\tau_{\text{tristimulus}} ::= \tau_{\text{XYZ}} \mid \tau_{\text{LMS}} \mid \tau_{\text{sRGB}}$ |
| Spectral types | $\tau_{\text{spectrum}} ::= \tau_{\text{Light}} \mid \tau_{\text{Reflectance}}$ |
| Physical types | $\tau ::= \tau_{\text{tristimulus}} \mid \tau_{\text{spectrum}}$ |
| Shaped types | $s ::= (\tau, d)$ |
| Values | $v ::= \tau(\alpha) \mid \tau(v) \mid v \oplus v$ |

Table 6: Augmented SmallerSpace syntax

$$\frac{\alpha : d \times \mathsf{channel\_count}(\tau)}{\tau(\alpha) : (\tau, d)} \ \text{Init}$$

$$\frac{v : (\tau_1, d) \qquad \mathsf{path\_exists}(\tau_1, \tau_2)}{\tau_2(v) : (\tau_2, d)} \ \text{Cast}$$

$$\frac{v_1, v_2 : (\tau_{\text{tristimulus}}, d)}{v_1 + v_2 : (\tau_{\text{tristimulus}}, d)} \ \text{TristimulusAdd}$$

$$\frac{v_1, v_2 : (\tau_{\text{Light}}, d)}{v_1 + v_2 : (\tau_{\text{Light}}, d)} \ \text{LightAdd}$$

$$\frac{v_1 : (\tau_{\text{Light}}, d) \qquad v_2 : (\tau_{\text{Reflectance}}, d)}{v_1 \times v_2 : (\tau_{\text{Light}}, d)} \ \text{Reflect}$$

$$\frac{}{\mathsf{broadcastable}(d, d)} \ \text{TrivialBroadcast}$$

$$\frac{}{\mathsf{broadcastable}(1, d)} \ \text{ScalarBroadcast}$$

$$\frac{d_1 = d_2 \times d_3}{\mathsf{broadcastable}(d_3, d_1)} \ \text{SubsetBroadcast}$$

$$\frac{\alpha_1 : d_1 \qquad \alpha_2 : d_2 \qquad \mathsf{broadcastable}(d_2, d_1)}{(\alpha_1) \oplus (\alpha_2) : d_1} \ \text{ArrayBinOpL}$$

$$\frac{\alpha_1 : d_1 \qquad \alpha_2 : d_2 \qquad \mathsf{broadcastable}(d_1, d_2)}{(\alpha_1) \oplus (\alpha_2) : d_2} \ \text{ArrayBinOpR}$$

$$\frac{\alpha_1 : d_1 \times d_i \qquad \alpha_2 : d_i \times d_2}{\mathsf{matmul}(\alpha_1, \alpha_2) : d_1 \times d_2} \ \text{ArrayMatMul}$$

Figure 5: Augmented SmallerSpace type rules.

### 3.2 Evaluation Rules

We have defined rules for evaluating SmallerSpace expressions. These rules can be found in Fig. 6. These evaluation rules operate on **"basic values"** like $\tau_{\text{Light}}(a_1)$ and $\tau_{\text{XYZ}}(a_2)$. $a_1$ and $a_2$ are array literals. Basic values are significant, as they represent the most reduced version of a colorspace value. They are defined only by a physical type and an array literal. As such, they cannot be evaluated any further. We will utilize $v_B$ to indicate the set of all basic values.

$$\tau_{\text{Light}}(a_1) + \tau_{\text{Light}}(a_2) \to \tau_{\text{Light}}((a_1) + (a_2)) \qquad \text{E-LightAdd}$$

$$\tau_{\text{XYZ}}(a_1) + \tau_{\text{XYZ}}(a_2) \to \tau_{\text{XYZ}}((a_1) + (a_2)) \qquad \text{E-XYZAdd}$$

$$\tau_{\text{LMS}}(a_1) + \tau_{\text{LMS}}(a_2) \to \tau_{\text{LMS}}((a_1) + (a_2)) \qquad \text{E-LMSAdd}$$

$$\tau_{\text{sRGB}}(a_1) + \tau_{\text{sRGB}}(a_2) \to$$
$$\tau_{\text{sRGB}}((((((a_1)/([255])) ** (\gamma_{\tau_{\text{sRGB}}})) + (((a_2)/([255])) ** ((\gamma_{\tau_{\text{sRGB}}})))) ** (\gamma^{-1}_{\tau_{\text{sRGB}}})) \times ([255])) \qquad \text{E-sRGBAdd}$$

$$\tau_{\text{Light}}(a_1) \times \tau_{\text{Reflectance}}(a_2) \to \tau_{\text{Light}}((a_1) \times (a_2)) \qquad \text{E-Reflect}$$

Figure 6: Evaluation rule for SmallerSpace type rules. $\gamma_{\tau_{\text{sRGB}}}$ and $\gamma^{-1}_{\tau_{\text{sRGB}}}$ are 1 dimension type array constants that represent the gamma value of the sRGB color space. They are 2.2 and $2.2^{-1}$, respectively.

We have several rules for evaluating castings. The rules listed in Fig. 7 represent edges in the casting graph (Fig. 1). In other words, they evaluate castings between adjacent types.

$$\tau_{\text{LMS}}(\tau_{\text{Light}}(a)) \to \tau_{\text{LMS}}(\mathsf{matmul}(a, M_{\text{Light2LMS}})) \qquad \text{E-Light2LMS}$$

$$\tau_{\text{LMS}}(\tau_{\text{XYZ}}(a)) \to \tau_{\text{LMS}}(\mathsf{matmul}(a, M_{\text{XYZ2LMS}})) \qquad \text{E-XYZ2LMS}$$

$$\tau_{\text{XYZ}}(\tau_{\text{LMS}}(a)) \to \tau_{\text{XYZ}}(\mathsf{matmul}(a, M_{\text{LMS2XYZ}})) \qquad \text{E-LMS2XYZ}$$

$$\tau_{\text{sRGB}}(\tau_{\text{XYZ}}(a)) \to \tau_{\text{sRGB}}((\mathsf{matmul}(a, M_{\text{XYZ2sRGB}})) ** (\gamma^{-1}_{\tau_{\text{sRGB}}})) \qquad \text{E-XYZ2sRGB}$$

$$\tau_{\text{XYZ}}(\tau_{\text{sRGB}}(a)) \to \tau_{\text{XYZ}}(\mathsf{matmul}((a) ** (\gamma_{\tau_{\text{sRGB}}}), M_{\text{sRGB2XYZ}})) \qquad \text{E-sRGB2XYZ}$$

Figure 7: Adjacent casting rules. The $M$ values represent array literal constants. All $M$ values with the exception of $M_{\text{XYZ2LMS}}$ are of dimension $3 \times 3$. $M_{\text{XYZ2LMS}}$ is of dimension $89 \times 3$

However, SmallerSpace also allows casting between types that are not adjacent on the casting graph. In order to achieve this, we have defined an additional function: $\mathsf{distance}(\tau_1, \tau_2)$ returns the number of edges in the shortest path from $\tau_1$ to $\tau_2$. We also define E-CastHop to evaluate casts between non-adjacent types.

$$\frac{\mathsf{path\_exists}(\tau_o, \tau_d) \qquad 1 \le \mathsf{distance}(\tau_i, \tau_d) < \mathsf{distance}(\tau_o, \tau_d) \qquad \mathsf{distance}(\tau_o, \tau_i) = 1}{\tau_d(\tau_o(a)) \to \tau_d(\tau_i(\tau_o(a)))} \ \text{E-CastHop}$$

We also need to account for castings from a type to itself. We design the E-CastTrivial evaluation relation for this purpose.

$$\tau(\tau(v)) \to \tau(v) \qquad \text{E-CastTrivial}$$

E-PropBinOpL and E-PropBinOpR allow an evaluation step to be taken on a binary operation if either operand can be further evaluated. E-PropCast does the same for casts. E-PropInit fulfills a similar function for nested array expressions that can be further evaluated.

$$\frac{v_1 \to v_1'}{v_1 \oplus v_2 \to v_1' \oplus v_2} \ \text{E-PropBinOpL}$$

$$\frac{v_2 \to v_2'}{v_1 \oplus v_2 \to v_1 \oplus v_2'} \ \text{E-PropBinOpR}$$

$$\frac{v \rightarrow v'}{\tau(v) \rightarrow \tau(v')} \text{ E-PropCast}$$

$$\frac{\alpha \rightarrow \alpha'}{\tau(\alpha) \rightarrow \tau(\alpha')} \text{ E-PropInit}$$

Since we have augmented SmallerSpace with array expressions, we also need rules to evaluate those, namely E-ArrBinOpL, E-ArrBinOpR, and E-ArrMatMul. These evaluation rules do not manipulate array literals, as array literals are abstracted in SmallerSpace. Instead, these evaluation rules utilize dimension type information to check if the evaluation is possible.

$$\frac{\alpha_1 : d_1 \qquad \alpha_2 : d_2 \qquad \alpha_1, \alpha_2 \in \mathbb{A} \qquad \mathsf{broadcastable}(d_2, d_1)}{\exists a_3 : d_1 \mid (\alpha_1) \oplus (\alpha_2) \rightarrow a_3} \text{ E-ArrBinOpL}$$

$$\frac{\alpha_1 : d_1 \qquad \alpha_2 : d_2 \qquad \alpha_1, \alpha_2 \in \mathbb{A} \qquad \mathsf{broadcastable}(d_1, d_2)}{\exists a_3 : d_2 \mid (\alpha_1) \oplus (\alpha_2) \rightarrow a_3} \text{ E-ArrBinOpR}$$

$$\frac{\alpha_1 : d_1 \times d_m \qquad \alpha_2 : d_m \times d_2 \qquad \alpha_1, \alpha_2 \in \mathbb{A}}{\exists a_3 : d_1 \times d_2 \mid \mathsf{matmul}(\alpha_1, \alpha_2) \rightarrow a_3} \text{ E-ArrMatMul}$$

We also need evaluation step propagation rules for array expressions as well.

$$\frac{\alpha_1 \rightarrow \alpha_1'}{(\alpha_1) \oplus (\alpha_2) \rightarrow (\alpha_1') \oplus (\alpha_2)} \text{ E-PropArrBinOpL}$$

$$\frac{\alpha_2 \rightarrow \alpha_2'}{(\alpha_1) \oplus (\alpha_2) \rightarrow (\alpha_1) \oplus (\alpha_2')} \text{ E-PropArrBinOpR}$$

$$\frac{\alpha_1 \rightarrow \alpha_1'}{\mathsf{matmul}(\alpha_1, \alpha_2) \rightarrow \mathsf{matmul}(\alpha_1', \alpha_2)} \text{ E-PropArrMatMulL}$$

$$\frac{\alpha_2 \rightarrow \alpha_2'}{\mathsf{matmul}(\alpha_1, \alpha_2) \rightarrow \mathsf{matmul}(\alpha_1, \alpha_2')} \text{ E-PropArrMatMulR}$$

# 4 Type Soundness Proof

We will prove type soundness through individual proofs of progress and preservation. A "basic value" is a value of the form $\tau(a)$. Basic values are significant as they are composed of only a physical type and an array literal. They cannot be evaluated any further. We will use $v_B$ to indicate the set of all basic values.

We prove SMALLERSPACE is type sound by showing that SMALLERSPACE satisfies both progress and preservation. Our proof for progress can be found in Sec. 4.3. Our preservation proof is in Sec. 4.4. Since SMALLERSPACE satisfies both progress and preservation, SMALLERSPACE is type sound. In order to show that SMALLERSPACE is type sound, we first define a set of "converse rules" in Sec. 4.1. Then, we prove that SMALLERSPACE's new array expressions also satisfy type soundness in Sec. 4.2.

## 4.1 Converse Rules

Similar to our proof of translational soundness, we will also be utilizing converse rules to prove type soundness. These rules will be labeled as CONV-RULENAME. In this section, we will detail each converse rule we utilize in our proof, and explain why they are valid.

$$\frac{\tau(\alpha) : (\tau, d)}{\alpha : d \times \mathsf{channel\_count}(\tau)}\ \textsc{Conv-Init}$$

The CONV-INIT type rule is the converse rule for the INIT type rule. CONV-INIT is valid because the INIT rule is the only rule that type checks values of the form $\tau(\alpha)$.

$$\frac{v : (\tau, d) \qquad v \in v_B}{\exists a : d \times \mathsf{channel\_count}(\tau) \mid v = \tau(a)}\ \textsc{Conv-BasicInit}$$

CONV-BASICINIT represents an alternative converse rule for the INIT type rule. CONV-BASICINIT is valid as if $v$ is a basic type, we know $v$ must take the form of $\tau(a)$, where $a$ is an array literal. Therefore, we can apply CONV-INIT to derive the dimension type of $a$.

$$\frac{v_1 + v_2 : (\tau_{\text{tristimulus}}, d)}{v_1, v_2 : (\tau_{\text{tristimulus}}, d)}\ \textsc{Conv-TristimulusAdd}$$

$$\frac{v_1 + v_2 : (\tau_{\text{Light}}, d)}{v_1, v_2 : (\tau_{\text{Light}}, d)}\ \textsc{Conv-LightAdd}$$

$$\frac{v_1 \times v_2 : (\tau_{\text{Light}}, d)}{v_1 : (\tau_{\text{Light}}, d) \wedge v_2 : (\tau_{\text{Light}}, d)}\ \textsc{Conv-Reflect}$$

$$\frac{\tau_2(v) : (\tau_2, d)}{\exists \tau_1 \mid v : (\tau_1, d) \wedge \mathsf{path\_exists}(\tau_1, \tau_2)}\ \textsc{Conv-Cast}$$

$$\frac{\mathsf{matmul}(\alpha_1, \alpha_2) : d}{\exists d_1, d_2, d_i \mid d = d_1 \times d_2 \wedge \alpha_1 : d_1 \times d_i \wedge \alpha_2 : d_i \times d_2}\ \textsc{Conv-ArrayMatMul}$$

CONV-TRISTIMULUSADD, CONV-LIGHTADD, CONV-REFLECT, CONV-CAST, and CONV-ARRAYMATMUL are inverted rules corresponding to the TRISTIMULUSADD, LIGHTADD, REFLECT, CAST, and ARRAYMATMUL rules. These converse rules are valid as TRISTIMULUSADD, LIGHTADD, REFLECT, CAST, and ARRAYMATMUL are the only rules that are able to type check $v_1 + v_2 : (\tau_{\text{tristimulus}}, d)$, $v_1 + v_2 : (\tau_{\text{Light}}, d)$, $v_1 \times v_2 : (\tau_{\text{Light}}, d)$, $\tau_2(v) : (\tau_2, d)$, and $\mathsf{matmul}(\alpha_1, \alpha_2) : d_1 \times d_2$.

$$\frac{(\alpha_1) \oplus (\alpha_2) : d}{(\exists d_1 \mid \alpha_1 : d_1 \wedge \alpha_2 : d \wedge \mathsf{broadcastable}(d_1, d)) \vee (\exists d_2 \mid \alpha_2 : d_2 \wedge \alpha_1 : d \wedge \mathsf{broadcastable}(d_2, d))}\ \textsc{Conv-ArrBinOp}$$

$$\frac{(\alpha_1) \oplus (\alpha_2) : d}{\exists d_1 \mid \alpha_1 : d_1 \wedge \alpha_2 : d \wedge \mathsf{broadcastable}(d_1, d)}\ \textsc{Conv-ArrBinOpL}$$

$$\frac{(\alpha_1) \oplus (\alpha_2) : d}{\exists d_2 \mid \alpha_2 : d_2 \wedge \alpha_1 : d \wedge \mathsf{broadcastable}(d_2, d)}\ \textsc{Conv-ArrBinOpR}$$

Since there are two rules that can type check the expression $(\alpha_1) \oplus (\alpha_2)$ (ARRAYBINOPL and ARRAYBINOPR), there are two disjoint conclusions that can be drawn from $(\alpha_1) \oplus (\alpha_2) : d$. At least one of the conclusions must be true. We split CONV-ARRBINOP into two individual rules for ease of use: CONV-ARRBINOPL and CONV-ARRBINOPR. These two rules are **not valid in isolation**. Every proof case that uses the CONV-ARRBINOPL type rule must also show that their conclusion holds when the CONV-ARRBINOPR type rule is used instead (and vice versa).

## 4.2 Array Expressions Type Soundness

Before we can prove the type soundness of SmallerSpace, we must first prove that array expressions are type sound. In order to do this, we must show that array expressions satisfy both progress and preservation.

### 4.2.1 Array Expressions Progress

**Theorem.** A typed array expression $\alpha$ is either an array literal ($\alpha \in \mathbb{A}$) or can take an evaluation step to some $\alpha'$. The theorem is formally stated below:

$$\frac{\alpha \notin \mathbb{A} \qquad \alpha : d}{\exists \alpha' \mid \alpha \to \alpha'} \text{ Array-Progress}$$

The progress theorem is paired with the following inductive hypothesis:

$$\frac{\alpha_i \subset \alpha \qquad \alpha_i \notin \mathbb{A} \qquad \alpha : d}{\exists \alpha_i' \mid \alpha_i \to \alpha_i'} \text{ Array-ProgHyp}$$

We will demonstrate that array expressions satisfy the progress theorem through proof by induction.

**Case 1: $\alpha \in \mathbb{A}$.** If $\alpha \in \mathbb{A}$, $\alpha$ is an array literal already and does not need to be further evaluated. The progress theorem holds for case 1.

**Case 2: $\alpha = (\alpha_1) \oplus (\alpha_2)$ and $\alpha_1 \notin \mathbb{A}$.**

$$\frac{\dfrac{\alpha_1 \subset (\alpha_1) \oplus (\alpha_2) \qquad \alpha_1 \notin \mathbb{A} \qquad (\alpha_1) \oplus (\alpha_2) : d}{\exists \alpha_1' \mid \alpha_1 \to \alpha_1'} \text{ Array-ProgHyp}}{\exists \alpha_1' \mid (\alpha_1) \oplus (\alpha_2) \to (\alpha_1') \oplus (\alpha_2)} \text{ E-PropArrBinOpL}$$

Since $(\alpha_1) \oplus (\alpha_2)$ can be further evaluated to $(\alpha_1') \oplus (\alpha_2)$, progress holds for this case.

**Case 3: $\alpha = (\alpha_1) \oplus (\alpha_2)$ and $\alpha_2 \notin \mathbb{A}$.** Similar to case 2.

$$\frac{\dfrac{\alpha_1 \subset (\alpha_1) \oplus (\alpha_2) \qquad \alpha_2 \notin \mathbb{A} \qquad (\alpha_1) \oplus (\alpha_2) : d}{\exists \alpha_2' \mid \alpha_2 \to \alpha_2'} \text{ Array-ProgHyp}}{\exists \alpha_2' \mid (\alpha_1) \oplus (\alpha_2) \to (\alpha_1) \oplus (\alpha_2')} \text{ E-PropArrBinOpR}$$

Since $(\alpha_1) \oplus (\alpha_2)$ can be further evaluated to $(\alpha_1) \oplus (\alpha_2')$, progress holds for this case.

**Case 4: $\alpha = (\alpha_1) \oplus (\alpha_2)$ and $\alpha_1, \alpha_2 \in \mathbb{A}$.**

$$\frac{\dfrac{(\alpha_1) \oplus (\alpha_2) : d}{\exists d_1 \mid \alpha_1 : d_1 \land \alpha_2 : d \land \mathsf{broadcastable}(d_1, d)} \text{ Conv-ArrBinOpL} \qquad \alpha_1, \alpha_2 \in \mathbb{A}}{\exists a_3 : d \mid (\alpha_1) \oplus (\alpha_2) \to a_3} \text{ E-ArrBinOpR}$$

Since Conv-ArrBinOpL is used in the above proof, we must also show that the conclusion holds when Conv-ArrBinOpR is used instead.

$$\frac{\dfrac{(\alpha_1) \oplus (\alpha_2) : d}{\exists d_2 \mid \alpha_2 : d_2 \land \alpha_1 : d \land \mathsf{broadcastable}(d_2, d)} \text{ Conv-ArrBinOpR} \qquad \alpha_1, \alpha_2 \in \mathbb{A}}{\exists a_3 : d \mid (\alpha_1) \oplus (\alpha_2) \to a_3} \text{ E-ArrBinOpL}$$

Regardless of whether Conv-ArrBinOpL or Conv-ArrBinOpR is used, we have shown that $(\alpha_1) \oplus (\alpha_2)$ evaluates to some $a_3 : d$ in this case. Therefore, progress holds for this case.

**Case 5:** $\alpha = \textbf{matmul}(\alpha_1, \alpha_2)$ **and** $\alpha_1 \notin \mathbb{A}$**.**

$$\dfrac{\dfrac{\alpha_1 \subset \mathsf{matmul}(\alpha_1, \alpha_2) \qquad \alpha_1 \notin \mathbb{A} \qquad \mathsf{matmul}(\alpha_1, \alpha_2) : d}{\exists \alpha_1' \mid \alpha_1 \to \alpha_1'}\ \textsc{Array-ProgHyp}}{\exists \alpha_1' \mid \mathsf{matmul}(\alpha_1, \alpha_2) \to \mathsf{matmul}(\alpha_1', \alpha_2)}\ \textsc{E-PropArrMatMulL}$$

Since $\mathsf{matmul}(\alpha_1, \alpha_2)$ evaluates to $\mathsf{matmul}(\alpha_1', \alpha_2)$, progress holds for this case.

**Case 6:** $\alpha = \textbf{matmul}(\alpha_1, \alpha_2)$ **and** $\alpha_2 \notin \mathbb{A}$**.**

$$\dfrac{\dfrac{\alpha_2 \subset \mathsf{matmul}(\alpha_1, \alpha_2) \qquad \alpha_2 \notin \mathbb{A} \qquad \mathsf{matmul}(\alpha_1, \alpha_2) : d}{\exists \alpha_2' \mid \alpha_2 \to \alpha_2'}\ \textsc{Array-ProgHyp}}{\exists \alpha_2' \mid \mathsf{matmul}(\alpha_1, \alpha_2) \to \mathsf{matmul}(\alpha_1, \alpha_2')}\ \textsc{E-PropArrMatMulR}$$

Since $\mathsf{matmul}(\alpha_1, \alpha_2)$ evaluates to $\mathsf{matmul}(\alpha_1, \alpha_2')$, progress holds for this case.

**Case 7:** $\alpha = \textbf{matmul}(\alpha_1, \alpha_2)$ **and** $\alpha_1, \alpha_2 \in \mathbb{A}$**.**

$$\dfrac{\dfrac{\mathsf{matmul}(\alpha_1, \alpha_2) : d}{\exists d_1, d_2, d_i | d = d_1 \times d_2 \land \alpha_1 : d_1 \times d_i \land \alpha_2 : d_i \times d_2}\ \textsc{Conv-ArrayMatMul} \qquad \alpha_1, \alpha_2 \in \mathbb{A}}{\exists a_3 : d_1 \times d_2 \mid \mathsf{matmul}(\alpha_1, \alpha_2) \to a_3}\ \textsc{E-ArrMatMul}$$

Since $\mathsf{matmul}(\alpha_1, \alpha_2)$ evaluates to some $a_3 : d_1 \times d_2$, progress holds for this case.

**Summary.** The seven cases that we prove progress for are comprehensive. In each case, we show that the corresponding array expression can take an evaluation step given the inductive hypothesis. Therefore, we have shown that the progress theorem holds for array expressions.

### 4.2.2 Array Expression Preservation

**Theorem.** A typed array expression $\alpha$ preserves its type after taking an evaluation step to $\alpha'$. The theorem is formally stated below:

$$\dfrac{\alpha : d \qquad \alpha \to \alpha'}{\alpha' : d}\ \textsc{Array-Preservation}$$

The preservation theorem is paired with the following inductive hypothesis:

$$\dfrac{\alpha_i \subset \alpha \qquad \alpha_i \to \alpha_i' \qquad \alpha_i : d}{\alpha_i' : d}\ \textsc{Array-PresHyp}$$

We will demonstrate that array expressions satisfy the preservation theorem through proof by structural induction. We will utilize the same cases that we utilized in the progress proof for array expressions.

**Case 1:** $\alpha \in \mathbb{A}$**.** If $\alpha \in \mathbb{A}$, $\alpha$ is an array literal already and cannot be evaluated further. Therefore, the preservation theorem does not apply.

**Case 2:** $\alpha = (\alpha_1) \oplus (\alpha_2)$ **and** $\alpha_1 \notin \mathbb{A}$**.**

$$\dfrac{\dfrac{\alpha_1 \notin \mathbb{A} \qquad \dfrac{(\alpha_1) \oplus (\alpha_2) : d}{\exists d_1 \mid \alpha_1 : d_1 \land \alpha_2 : d \land \mathsf{broadcastable}(d_1, d)}\ \textsc{Conv-ArrBinOpL}}{\exists \alpha_1' \mid \alpha_1 \to \alpha_1'}\ \textsc{Array-Progress}}{\exists \alpha_1' \mid (\alpha_1) \oplus (\alpha_2) \to (\alpha_1') \oplus (\alpha_2)}\ \textsc{E-PropArrBinOpL}$$

$$\dfrac{\alpha_2 : d \qquad \exists d_1 \mid \mathsf{broadcastable}(d_1, d) \qquad \dfrac{\alpha_1 \subset (\alpha_1) \oplus (\alpha_2) \qquad \exists \alpha_1' \mid \alpha_1 \to \alpha_1' \qquad \exists d_1 \mid \alpha_1 : d_1}{\exists \alpha_1', d_1 \mid \alpha_1' : d_1}\ \textsc{Array-PresHyp}}{\exists \alpha_1' \mid (\alpha_1') \oplus (\alpha_2) : d}\ \textsc{ArrayBinOpR}$$

Since Conv-ArrBinOpL is used in the above proof, we must also show that the conclusion holds when Conv-ArrBinOpR is used instead.

$$\dfrac{\alpha_1 \notin \mathbb{A} \qquad \dfrac{(\alpha_1) \oplus (\alpha_2) : d}{\exists d_2 \mid \alpha_1 : d \wedge \alpha_2 : d_2 \wedge \mathsf{broadcastable}(d_2, d)}\ \textsc{Conv-ArrBinOpR}}{\dfrac{\exists \alpha_1' \mid \alpha_1 \to \alpha_1'}{\exists \alpha_1' \mid (\alpha_1) \oplus (\alpha_2) \to (\alpha_1') \oplus (\alpha_2)}\ \textsc{E-PropArrBinOpL}}\ \textsc{Array-Progress}$$

$$\dfrac{\exists d_2 \mid \alpha_2 : d_2 \qquad \exists d_2 \mid \mathsf{broadcastable}(d_2, d) \qquad \dfrac{\alpha_1 \subset (\alpha_1) \oplus (\alpha_2) \qquad \exists \alpha_1' \mid \alpha_1 \to \alpha_1' \qquad \alpha_1 : d}{\exists \alpha_1' \mid \alpha_1' : d}\ \textsc{Array-PresHyp}}{\exists \alpha_1' \mid (\alpha_1') \oplus (\alpha_2) : d}\ \textsc{ArrayBinOpL}$$

We have shown that $(\alpha_1) \oplus (\alpha_2) \to (\alpha_1') \oplus (\alpha_2)$ and $(\alpha_1') \oplus (\alpha_2) : d$. $(\alpha_1) \oplus (\alpha_2)$ also has the type $d$. Therefore, preservation is satisfied for this case.

**Case 3:** $\alpha = (\alpha_1) \oplus (\alpha_2)$ **and** $\alpha_2 \notin \mathbb{A}$**.** Similar to case 2.

$$\dfrac{\alpha_2 \notin \mathbb{A} \qquad \dfrac{(\alpha_1) \oplus (\alpha_2) : d}{\exists d_1 \mid \alpha_1 : d_1 \wedge \alpha_2 : d \wedge \mathsf{broadcastable}(d_1, d)}\ \textsc{Conv-ArrBinOpL}}{\dfrac{\exists \alpha_2' \mid \alpha_2 \to \alpha_2'}{\exists \alpha_2' \mid (\alpha_1) \oplus (\alpha_2) \to (\alpha_1) \oplus (\alpha_2')}\ \textsc{E-PropArrBinOpR}}\ \textsc{Array-Progress}$$

$$\dfrac{\exists d_1 \mid \alpha_1 : d_1 \qquad \exists d_1 \mid \mathsf{broadcastable}(d_1, d) \qquad \dfrac{\alpha_2 \subset (\alpha_1) \oplus (\alpha_2) \qquad \exists \alpha_2' \mid \alpha_2 \to \alpha_2' \qquad \alpha_2 : d}{\exists \alpha_2' \mid \alpha_2' : d}\ \textsc{Array-PresHyp}}{\exists \alpha_2' \mid (\alpha_1) \oplus (\alpha_2') : d}\ \textsc{ArrayBinOpR}$$

Since Conv-ArrBinOpL is used in the above proof, we must also show that the conclusion holds when Conv-ArrBinOpR is used instead.

$$\dfrac{\alpha_2 \notin \mathbb{A} \qquad \dfrac{(\alpha_1) \oplus (\alpha_2) : d}{\exists d_2 \mid \alpha_1 : d \wedge \alpha_2 : d_2 \wedge \mathsf{broadcastable}(d_2, d)}\ \textsc{Conv-ArrBinOpR}}{\dfrac{\exists \alpha_2' \mid \alpha_2 \to \alpha_2'}{\exists \alpha_2' \mid (\alpha_1) \oplus (\alpha_2) \to (\alpha_1) \oplus (\alpha_2')}\ \textsc{E-PropArrBinOpR}}\ \textsc{Array-Progress}$$

$$\dfrac{\alpha_1 : d \qquad \exists d_2 \mid \mathsf{broadcastable}(d_2, d) \qquad \dfrac{\alpha_2 \subset (\alpha_1) \oplus (\alpha_2) \qquad \exists \alpha_2' \mid \alpha_2 \to \alpha_2' \qquad \alpha_2 : d}{\exists \alpha_2', d_2 \mid \alpha_2' : d_2}\ \textsc{Array-PresHyp}}{\exists \alpha_2' \mid (\alpha_1) \oplus (\alpha_2') : d}\ \textsc{ArrayBinOpL}$$

We have shown that $(\alpha_1) \oplus (\alpha_2) \to (\alpha_1) \oplus (\alpha_2')$ and $(\alpha_1) \oplus (\alpha_2') : d$. $(\alpha_1) \oplus (\alpha_2)$ also has the type $d$. Therefore, preservation is satisfied for this case.

**Case 4:** $\alpha = (\alpha_1) \oplus (\alpha_2)$ **and** $\alpha_1, \alpha_2 \in \mathbb{A}$**.** We know from case 4 of the progress proof that $(\alpha_1) \oplus (\alpha_2) \to a_3$ and that $a_3 : d$. Since $(\alpha_1) \oplus (\alpha_2)$ also has the dimension $d$, the preservation theorem is satisfied for this case.

**Case 5:** $\alpha = \mathbf{matmul}(\alpha_1, \alpha_2)$ **and** $\alpha_1 \notin \mathbb{A}$**.**

$$\dfrac{\alpha_1 \notin \mathbb{A} \qquad \dfrac{\mathsf{matmul}(\alpha_1, \alpha_2) : d}{\exists d_1, d_2, d_i \mid d = d_1 \times d_2 \wedge \alpha_1 : d_1 \times d_i \wedge \alpha_2 : d_i \times d_2}\ \textsc{Conv-ArrayMatMul}}{\dfrac{\exists \alpha_1' \mid \alpha_1 \to \alpha_1'}{\exists \alpha_1' \mid \mathsf{matmul}(\alpha_1, \alpha_2) \to \mathsf{matmul}(\alpha_1', \alpha_2)}\ \textsc{E-PropArrMatMulL}}\ \textsc{ArrayProgress}$$

$$\dfrac{\exists d_1, d_2 \mid d = d_1 \times d_2 \qquad \dfrac{\exists d_i, d_2 \mid \alpha_2 : d_i \times d_2 \qquad \dfrac{\alpha_1 \in \mathsf{matmul}(\alpha_1, \alpha_2) \qquad \exists \alpha_1' \mid \alpha_1 \to \alpha_1' \qquad \exists d_1, d_i \mid \alpha_1 : d_1 \times d_i}{\exists \alpha_1', d_1, d_i \mid \alpha_1' : d_1 \times d_i}\ \textsc{Array-PresHyp}}{\exists \alpha_1', d_1, d_2 \mid \mathsf{matmul}(\alpha_1', \alpha_2) : d_1 \times d_2}\ \textsc{ArrayMatMul}}{\exists \alpha_1' \mid \mathsf{matmul}(\alpha_1', \alpha_2) : d}\ \textsc{Subst}$$

Since $\mathsf{matmul}(\alpha_1, \alpha_2) : d$, $\mathsf{matmul}(\alpha_1, \alpha_2) \to \mathsf{matmul}(\alpha_1', \alpha_2)$, and $\mathsf{matmul}(\alpha_1', \alpha_2) : d$, preservation holds for this case.

**Case 6:** $\alpha = \textsf{\textbf{matmul}}(\alpha_1, \alpha_2)$ **and** $\alpha_2 \notin \mathbb{A}$**.**

$$
\dfrac{\dfrac{\alpha_2 \notin \mathbb{A} \qquad \dfrac{\textsf{matmul}(\alpha_1, \alpha_2) : d}{\exists d_1, d_2, d_i \mid d = d_1 \times d_2 \wedge \alpha_1 : d_1 \times d_i \wedge \alpha_2 : d_i \times d_2}\ \textsc{Conv-ArrayMatMul}}{\exists \alpha_2' \mid \alpha_2 \rightarrow \alpha_2'}\ \textsc{Array-Progress}}{\exists \alpha_2' \mid \textsf{matmul}(\alpha_1, \alpha_2) \rightarrow \textsf{matmul}(\alpha_1, \alpha_2')}\ \textsc{E-PropArrMatMulL}
$$

$$
\dfrac{\exists d_1, d_2 \mid d = d_1 \times d_2 \qquad \dfrac{\exists d_1, d_i \mid \alpha_1 : d_1 \times d_i \qquad \dfrac{\alpha_2 \in \textsf{matmul}(\alpha_1, \alpha_2) \quad \exists \alpha_2' \mid \alpha_2 \rightarrow \alpha_2' \quad \exists d_2, d_i \mid \alpha_2 : d_i \times d_2}{\exists \alpha_2', d_2, d_i \mid \alpha_2' : d_i \times d_2}\ \textsc{Array-PresHyp}}{\exists \alpha_2', d_1, d_2 \mid \textsf{matmul}(\alpha_1, \alpha_2') : d_1 \times d_2}\ \textsc{ArrayMatMul}}{\exists \alpha_2' \mid \textsf{matmul}(\alpha_1, \alpha_2') : d}\ \textsc{Subst}
$$

Since $\textsf{matmul}(\alpha_1, \alpha_2) : d$, $\textsf{matmul}(\alpha_1, \alpha_2) \rightarrow \textsf{matmul}(\alpha_1, \alpha_2')$, and $\textsf{matmul}(\alpha_1, \alpha_2') : d$, preservation holds for this case.

**Case 7:** $\alpha = \textsf{\textbf{matmul}}(\alpha_1, \alpha_2)$ **and** $\alpha_1, \alpha_2 \in \mathbb{A}$**.** In case 7 of the progress proof, we showed that $\textsf{matmul}(\alpha_1, \alpha_2) \rightarrow \alpha_3$, and that $\alpha_3 : d_1 \times d_2$. We also showed that $d = d_1 \times d_2$. Therefore, $\alpha_3 : d$. Since $\textsf{matmul}(\alpha_1, \alpha_2) : d$, $\textsf{matmul}(\alpha_1, \alpha_2) \rightarrow \alpha_3$, and $\alpha_3 : d$, preservation holds for this case.

**Summary.** The seven cases that we prove preservation for are comprehensive. In each case, we show that, if the corresponding array expression can be evaluated further, the type of the array expression remains unchanged after evaluation. The preservation theorem holds for array expressions.

## 4.3 Progress

**Theorem.** A typed value $v$ is either a basic value of the form $\tau(a)$ or can take an evaluation step to some $v'$. The theorem is more formally stated below:

$$\frac{v \notin v_B \qquad v : (\tau, d)}{\exists v' \mid v \to v'}\ \textsc{Progress}$$

We will utilize structural induction to prove the progress theorem. Our inductive hypothesis is as follows:

$$\frac{v_i \subset v \qquad v_i \notin v_B \qquad v : (\tau, d)}{\exists v'_i \mid v_i \to v'_i}\ \textsc{Prog-IndHyp}$$

We will show that the theorem of progress holds for each SmallerSpace rule that can type check a value.

### 4.3.1 Init Progress

$$\frac{\alpha : d \times \mathsf{channel\_count}(\tau)}{\tau(\alpha) : (\tau, d)}\ \textsc{Init}$$

**Case 1: $\alpha \in \mathbb{A}$.** If $\alpha$ is an array literal, $\tau(\alpha)$ is a basic value and cannot be evaluated further. Therefore, the progress theorem holds for this case.

**Case 2: $\alpha \notin \mathbb{A}$.** We have proven Array-Progress. As such, we know that if $\alpha \notin \mathbb{A}$, there must exist some $\alpha'$ such that $\alpha \to \alpha'$. Through E-PropInit, we can conlude that $\tau(\alpha) \to \tau(\alpha')$. Therefore, Value-Progress holds for case 2.

**Summary.** Since the progress theorem holds for all cases of the Init rule, the Init rule satisfies the progress theorem. Any non-basic value that is type checked by the Init rule can be further evaluated.

### 4.3.2 Cast Progress

$$\frac{v : (\tau_1, d) \qquad \mathsf{path\_exists}(\tau_1, \tau_2)}{\tau_2(v) : (\tau_2, d)}\ \textsc{Cast}$$

**Case 1: $v \notin v_B$.** If $v \notin v_B$, we can conclude by the inductive hypothesis and E-PropCast that there exists some $v'$ such that $\tau_2(v) \to \tau_2(v')$.

**Case 2: $v \in v_B$, $\tau_1 = \tau_2$.**

$$\cfrac{\cfrac{v \in v_B \quad \cfrac{\tau_2(v) : (\tau_2, d)}{\exists \tau_1 \mid v : (\tau_1, d)}\ \textsc{Conv-Cast}}{\exists \tau_1, a_1 : d \times \mathsf{channel\_count}(\tau_1) \mid v = \tau_1(a_1)}\ \textsc{Conv-BasicInit} \quad \cfrac{\tau_1 = \tau_2 \quad \cfrac{}{\tau_1(\tau_1(a_1)) \to \tau_1(a_1)}\ \textsc{E-CastTrivial}}{\tau_2(\tau_1(a_1)) \to \tau_2(a_1)}\ \textsc{Subst}}{\exists \tau_1, a_1 : d \times \mathsf{channel\_count}(\tau_1) \mid \tau_2(v) \to \tau_2(a_1)}\ \textsc{Subst}$$

Since $\tau_2(v) \to \tau_2(a_1)$, progress is fulfilled for this case.

**Case 3: $v \in v_B$, $\tau_1$ adjacent to $\tau_2$.** If $\tau_1$ and $\tau_2$ are adjacent in the casting graph and $\mathsf{path\_exists}(\tau_1, \tau_2)$, there exists a corresponding adjacent casting rule. A list of these rules can be found in Fig. 7. We can apply these rules to show that there exists some $\alpha$ such that $\tau_2(v) \to \tau_2(\alpha)$. This shows that Value-Progress holds for this case. We will show one example of this case, where $\tau_1 = \tau_{\text{Light}}$ and $\tau_2 = \tau_{\text{LMS}}$:

$$\cfrac{\cfrac{v \in v_B \quad \cfrac{\tau_1 = \tau_{\text{Light}} \quad \cfrac{\tau_2(v) : (\tau_2, d)}{\exists \tau_1 \mid v : (\tau_1, d)}\ \textsc{Conv-Cast}}{v : (\tau_{\text{Light}}, d)}\ \textsc{Subst}}{\exists a : d \times \mathsf{channel\_count}(\tau_{\text{Light}}) \mid v = \tau_{\text{Light}}(a)}\ \textsc{Conv-BasicInit} \quad \cfrac{\tau_2 = \tau_{\text{LMS}} \quad \cfrac{}{\tau_{\text{LMS}}(\tau_{\text{Light}}(a)) \to \tau_{\text{LMS}}(\mathsf{matmul}(a, M_{\textsc{Light2LMS}}))}\ \textsc{E-Light2LMS}}{\tau_2(\tau_{\text{Light}}(a)) \to \tau_2(\mathsf{matmul}(a, M_{\textsc{Light2LMS}}))}\ \textsc{Subst}}{\tau_2(v) \to \tau_2(\mathsf{matmul}(a, M_{\textsc{Light2LMS}}))}\ \textsc{Subst}$$

Since $\tau_2(v) \to \tau_2(\mathsf{matmul}(a, M_{\text{LIGHT2LMS}}))$, the progress theorem holds for this sub-case. Other instances of this case (i.e. $\tau_1 = \tau_{\text{XYZ}}$, $\tau_2 = \tau_{\text{sRGB}}$) come to the same conclusion.

**Case 4: $v \in v_B$, $\tau_1$ not adjacent to $\tau_2$.** From Conv-Cast, we know that $\mathsf{path\_exists}(\tau_1, \tau_2)$. We also know that in this case there is at least 1 hop that needs to be made between $\tau_1$ and $\tau_2$ on the casting graph. Since the casting graph is a directed forest, there is a unique shortest path between $\tau_1$ and $\tau_2$. Therefore, E-CastHop will be able to find some $\tau_i$ such that $\tau_2(v) \to \tau_2(\tau_i(v))$. We will show one example where $\tau_1 = \tau_{\text{Light}}$ and $\tau_2 = \tau_{\text{XYZ}}$:

$$\dfrac{\tau_2 = \tau_{\text{XYZ}} \qquad \dfrac{\mathsf{path\_exists}(\tau_{\text{Light}}, \tau_{\text{XYZ}}) \quad 1 \leq \mathsf{distance}(\tau_{\text{LMS}}, \tau_{\text{XYZ}}) \leq \mathsf{distance}(\tau_{\text{Light}}, \tau_{\text{XYZ}}) \quad \mathsf{distance}(\tau_{\text{Light}}, \tau_{\text{LMS}}) = 1}{\tau_{\text{XYZ}}(\tau_{\text{Light}}(a)) \to \tau_{\text{XYZ}}(\tau_{\text{LMS}}(\tau_{\text{Light}}(a)))}\ \textsc{E-CastHop}}{\tau_2(\tau_{\text{Light}}(a)) \to \tau_2(\tau_{\text{LMS}}(\tau_{\text{Light}}(a)))}\ \textsc{Subst}$$

$$\dfrac{\tau_2(\tau_{\text{Light}}(a)) \to \tau_2(\tau_{\text{LMS}}(\tau_{\text{Light}}(a))) \qquad \dfrac{v \in v_B \qquad \dfrac{\tau_1 = \tau_{\text{Light}} \qquad \dfrac{\tau_2(v) : (\tau_2, d)}{\exists \tau_1 \mid v : (\tau_1, d)}\ \textsc{Conv-Cast}}{v : (\tau_{\text{Light}}, d)}\ \textsc{Subst}}{\exists a \times \mathsf{channel\_count}(\tau_{\text{Light}}) \mid v = \tau_{\text{Light}}(a)}\ \textsc{Conv-BasicInit}}{\tau_2(v) \to \tau_2(\tau_{\text{LMS}}(v))}\ \textsc{Subst}$$

Since $\tau_2(v) \to \tau_2(\tau_{\text{LMS}}(v))$, the progress theorem holds for this sub-case. Other instances of this case (i.e. $\tau_1 = \tau_{\text{LMS}}$, $\tau_2 = \tau_{\text{sRGB}}$) come to the same conclusion.

**Summary.** Since the progress theorem holds for all cases of the Cast rule, the Cast rule satisfies the progress theorem. Any non-basic value that is type checked by the Cast rule can be further evaluated.

### 4.3.3 TristimulusAdd Progress

$$\dfrac{v_1, v_2 : (\tau_{\text{tristimulus}}, d)}{v_1 + v_2 : (\tau_{\text{tristimulus}}, d)}\ \textsc{TristimulusAdd}$$

**Case 1: $v_1 \notin v_B$ and/or $v_2 \notin v_B$.** By the inductive hypothesis, there must exist some $v_1'$ such that $v_1 \to v_1'$ or some $v_2'$ such that $v_2 \to v_2'$. By E-PropBinOpL or E-PropBinOpR, we can conclude that $v_1 + v_2 \to v_1' + v_2$ or $v_1 + v_2 \to v_1 + v_2'$. Therefore, progress holds for this case.

**Case 2: $v_1, v_2 \in v_B$.** We can see from the Conv-TristimulusAdd rule that both $v_1$ and $v_2$ must share the same shaped type. A different evaluation rule may apply to the value depending on what tristimulus type $v_1$ and $v_2$ share. We will exhaustively cover every possible tristimulus type case.

**Case 2-a:** $v_1, v_2 : (\tau_{\textbf{XYZ}}, d)$

$$\dfrac{v_1 \in v_B \qquad \dfrac{v_1 + v_2 : (\tau_{\text{XYZ}}, d)}{v_1 : (\tau_{\text{XYZ}}, d)}\ \textsc{Conv-TristimulusAdd}}{\exists a_1 : d \times \mathsf{channel\_count}(\tau_{\text{XYZ}}) \mid v_1 = \tau_{\text{XYZ}}(a_1)}\ \textsc{Conv-BasicInit}$$

$$\dfrac{v_2 \in v_B \qquad \dfrac{v_1 + v_2 : (\tau_{\text{XYZ}}, d)}{v_2 : (\tau_{\text{XYZ}}, d)}\ \textsc{Conv-TristimulusAdd}}{\exists a_2 : d \times \mathsf{channel\_count}(\tau_{\text{XYZ}}) \mid v_2 = \tau_{\text{XYZ}}(a_2)}\ \textsc{Conv-BasicInit}$$

$$\dfrac{\dfrac{}{\tau_{\text{XYZ}}(a_1) + \tau_{\text{XYZ}}(a_2) \to \tau_{\text{XYZ}}((a_1) + (a_2))}\ \textsc{E-XYZAdd} \qquad \exists a_1 : d \times \mathsf{channel\_count}(\tau_{\text{XYZ}}) \mid v_1 = \tau_{\text{XYZ}}(a_1)}{\exists a_1 : d \times \mathsf{channel\_count}(\tau_{\text{XYZ}}) \mid v_1 + \tau_{\text{XYZ}}(a_2) \to \tau_{\text{XYZ}}((a_1) + (a_2))}\ \textsc{Subst}$$

$$\dfrac{\exists a_1 : d \times \mathsf{channel\_count}(\tau_{\text{XYZ}}) \mid v_1 + \tau_{\text{XYZ}}(a_2) \to \tau_{\text{XYZ}}((a_1) + (a_2)) \qquad \exists a_2 : d \times \mathsf{channel\_count}(\tau_{\text{XYZ}}) \mid v_2 = \tau_{\text{XYZ}}(a_2)}{\exists a_1, a_2 : d \times \mathsf{channel\_count}(\tau_{\text{XYZ}}) \mid v_1 + v_2 \to \tau_{\text{XYZ}}((a_1) + (a_2))}\ \textsc{Subst}$$

Since $v_1 + v_2 \to \tau_{\text{XYZ}}((a_1) + (a_2))$, progress holds for this case.

**Case 2-b:** $v_1, v_2 : (\tau_{\mathbf{LMS}}, d)$

$$\frac{v_1 \in v_B \qquad \dfrac{v_1 + v_2 : (\tau_{\mathrm{LMS}}, d)}{v_1 : (\tau_{\mathrm{LMS}}, d)}\;\textsc{Conv-TristimulusAdd}}{\exists a_1 : d \times \mathsf{channel\_count}(\tau_{\mathrm{LMS}}) \mid v_1 = \tau_{\mathrm{LMS}}(a_1)}\;\textsc{Conv-BasicInit}$$

$$\frac{v_2 \in v_B \qquad \dfrac{v_1 + v_2 : (\tau_{\mathrm{LMS}}, d)}{v_2 : (\tau_{\mathrm{LMS}}, d)}\;\textsc{Conv-TristimulusAdd}}{\exists a_2 : d \times \mathsf{channel\_count}(\tau_{\mathrm{LMS}}) \mid v_2 = \tau_{\mathrm{LMS}}(a_2)}\;\textsc{Conv-BasicInit}$$

$$\frac{\dfrac{}{\tau_{\mathrm{LMS}}(a_1) + \tau_{\mathrm{LMS}}(a_2) \to \tau_{\mathrm{LMS}}((a_1) + (a_2))}\;\textsc{E-LMSAdd} \qquad \exists a_1 : d \times \mathsf{channel\_count}(\tau_{\mathrm{LMS}}) \mid v_1 = \tau_{\mathrm{LMS}}(a_1)}{\exists a_1 : d \times \mathsf{channel\_count}(\tau_{\mathrm{LMS}}) \mid v_1 + \tau_{\mathrm{LMS}}(a_2) \to \tau_{\mathrm{LMS}}((a_1) + (a_2))}\;\textsc{Subst}$$

$$\frac{\exists a_1 : d \times \mathsf{channel\_count}(\tau_{\mathrm{LMS}}) \mid v_1 + \tau_{\mathrm{LMS}}(a_2) \to \tau_{\mathrm{LMS}}((a_1) + (a_2)) \qquad \exists a_2 : d \times \mathsf{channel\_count}(\tau_{\mathrm{LMS}}) \mid v_2 = \tau_{\mathrm{LMS}}(a_2)}{\exists a_1, a_2 : d \times \mathsf{channel\_count}(\tau_{\mathrm{LMS}}) \mid v_1 + v_2 \to \tau_{\mathrm{LMS}}((a_1) + (a_2))}\;\textsc{Subst}$$

Since $v_1 + v_2 \to \tau_{\mathrm{LMS}}((a_1) + (a_2))$, progress holds for this case.

**Case 2-c:** $v_1, v_2 : (\tau_{\mathbf{sRGB}}, d)$

$$\frac{v_1 \in v_B \qquad \dfrac{v_1 + v_2 : (\tau_{\mathrm{sRGB}}, d)}{v_1 : (\tau_{\mathrm{sRGB}}, d)}\;\textsc{Conv-TristimulusAdd}}{\exists a_1 : d \times \mathsf{channel\_count}(\tau_{\mathrm{sRGB}}) \mid v_1 = \tau_{\mathrm{sRGB}}(a_1)}\;\textsc{Conv-BasicInit}$$

$$\frac{v_2 \in v_B \qquad \dfrac{v_1 + v_2 : (\tau_{\mathrm{sRGB}}, d)}{v_2 : (\tau_{\mathrm{sRGB}}, d)}\;\textsc{Conv-TristimulusAdd}}{\exists a_2 : d \times \mathsf{channel\_count}(\tau_{\mathrm{sRGB}}) \mid v_2 = \tau_{\mathrm{sRGB}}(a_2)}\;\textsc{Conv-BasicInit}$$

$$\frac{}{\tau_{\mathrm{sRGB}}(a_1) + \tau_{\mathrm{sRGB}}(a_2) \to \tau_{\mathrm{sRGB}}((((((a_1)/([255])) ** (\gamma_{\tau_{\mathrm{sRGB}}})) + (((a_2)/([255])) ** ((\gamma_{\tau_{\mathrm{sRGB}}})))) ** (\gamma^{-1}_{\tau_{\mathrm{sRGB}}})) \times ([255]))}\;\textsc{E-sRGBAdd}$$

$$\frac{v_1 : (\tau_{\mathrm{sRGB}}, d) \qquad \tau_{\mathrm{sRGB}}(a_1) + \tau_{\mathrm{sRGB}}(a_2) \to \tau_{\mathrm{sRGB}}((((((a_1)/([255])) ** (\gamma_{\tau_{\mathrm{sRGB}}})) + (((a_2)/([255])) ** ((\gamma_{\tau_{\mathrm{sRGB}}})))) ** (\gamma^{-1}_{\tau_{\mathrm{sRGB}}})) \times ([255]))}{\exists a_1 : d \times \mathsf{channel\_count}(\tau_{\mathrm{sRGB}}) \mid v_1 + \tau_{\mathrm{sRGB}}(a_2) \to \tau_{\mathrm{sRGB}}((((((a_1)/([255])) ** (\gamma_{\tau_{\mathrm{sRGB}}})) + (((a_2)/([255])) ** ((\gamma_{\tau_{\mathrm{sRGB}}})))) ** (\gamma^{-1}_{\tau_{\mathrm{sRGB}}})) \times ([255]))}\;\textsc{Subst}$$

$$\frac{v_2 : (\tau_{\mathrm{sRGB}}, d) \qquad v_1 + \tau_{\mathrm{sRGB}}(a_2) \to \tau_{\mathrm{sRGB}}((((((a_1)/([255])) ** (\gamma_{\tau_{\mathrm{sRGB}}})) + (((a_2)/([255])) ** ((\gamma_{\tau_{\mathrm{sRGB}}})))) ** (\gamma^{-1}_{\tau_{\mathrm{sRGB}}})) \times ([255]))}{\exists a_1, a_2 : d \times \mathsf{channel\_count}(\tau_{\mathrm{sRGB}}) \mid v_1 + v_2 \to \tau_{\mathrm{sRGB}}((((((a_1)/([255])) ** (\gamma_{\tau_{\mathrm{sRGB}}})) + (((a_2)/([255])) ** ((\gamma_{\tau_{\mathrm{sRGB}}})))) ** (\gamma^{-1}_{\tau_{\mathrm{sRGB}}})) \times ([255]))}\;\textsc{Subst}$$

Since $v_1 + v_2 \to \tau_{\mathrm{sRGB}}(...)$, progress holds for this case.

**Summary.** Since the progress theorem holds for all cases of the TristimulusAdd rule, the TristimulusAdd rule satisfies the progress theorem. Any non-basic value that is type checked by the TristimulusAdd rule can be further evaluated.

### 4.3.4 LightAdd Progress

$$\frac{v_1, v_2 : (\tau_{\mathrm{Light}}, d)}{v_1 + v_2 : (\tau_{\mathrm{Light}}, d)}\;\textsc{LightAdd}$$

**Case 1:** $v_1 \notin v_B$ **and/or** $v_2 \notin v_B$**.** By the inductive hypothesis, there must exist some $v_1'$ such that $v_1 \to v_1'$ or some $v_2'$ such that $v_2 \to v_2'$. By E-PropBinOpL or E-PropBinOpR, we can conclude that $v_1 + v_2 \to v_1' + v_2$ or $v_1 + v_2 \to v_1 + v_2'$. Therefore, progress holds for this case.

**Case 2:** $v_1, v_2 \in v_B$.

$$\dfrac{v_1 \in v_B \qquad \dfrac{v_1 + v_2 : (\tau_{\text{Light}}, d)}{v_1 : (\tau_{\text{Light}}, d)}\ \textsc{Conv-LightAdd}}{\exists a_1 : d \times \mathsf{channel\_count}(\tau_{\text{Light}}) \mid v_1 = \tau_{\text{Light}}(a_1)}\ \textsc{Conv-BasicInit}$$

$$\dfrac{v_2 \in v_B \qquad \dfrac{v_1 + v_2 : (\tau_{\text{Light}}, d)}{v_2 : (\tau_{\text{Light}}, d)}\ \textsc{Conv-LightAdd}}{\exists a_2 : d \times \mathsf{channel\_count}(\tau_{\text{Light}}) \mid v_2 = \tau_{\text{Light}}(a_2)}\ \textsc{Conv-BasicInit}$$

$$\dfrac{\dfrac{}{\tau_{\text{Light}}(a_1) + \tau_{\text{Light}}(a_2) \to \tau_{\text{Light}}((a_1) + (a_2))}\ \textsc{E-LightAdd} \qquad \exists a_1 : d \times \mathsf{channel\_count}(\tau_{\text{Light}}) \mid v_1 = \tau_{\text{Light}}(a_1)}{\exists a_1 : d \times \mathsf{channel\_count}(\tau_{\text{Light}}) \mid v_1 + \tau_{\text{Light}}(a_2) \to \tau_{\text{Light}}((a_1) + (a_2))}\ \textsc{Subst}$$

$$\dfrac{\exists a_1 : d \times \mathsf{channel\_count}(\tau_{\text{Light}}) \mid v_1 + \tau_{\text{Light}}(a_2) \to \tau_{\text{Light}}((a_1) + (a_2)) \qquad \exists a_2 : d \times \mathsf{channel\_count}(\tau_{\text{Light}}) \mid v_2 = \tau_{\text{Light}}(a_2)}{\exists a_1, a_2 : d \times \mathsf{channel\_count}(\tau_{\text{Light}}) \mid v_1 + v_2 \to \tau_{\text{Light}}((a_1) + (a_2))}\ \textsc{Subst}$$

Since $v_1 + v_2 \to \tau_{\text{Light}}((a_1) + (a_2))$, progress holds for this case.

**Summary.** Since the progress theorem holds for both cases of the LightAdd rule, the LightAdd rule satisfies the progress theorem. Any non-basic value that is type checked by the LightAdd rule can be further evaluated.

### 4.3.5 Reflect Progress

$$\dfrac{v_1 : (\tau_{\text{Light}}, d) \qquad v_2 : (\tau_{\text{Reflectance}}, d)}{v_1 \times v_2 : (\tau_{\text{Light}}, d)}\ \textsc{Reflect}$$

**Case 1:** $v_1 \notin v_B$ **and/or** $v_2 \notin v_B$. By the inductive hypothesis, there must exist some $v_1'$ such that $v_1 \to v_1'$ or some $v_2'$ such that $v_2 \to v_2'$. By E-PropBinOpL or E-PropBinOpR, we can conclude that $v_1 \times v_2 \to v_1' \times v_2$ or $v_1 \times v_2 \to v_1 \times v_2'$. Therefore, progress holds for this case.

**Case 2:** $v_1, v_2 \notin v_B$.

$$\dfrac{v_1 \in v_B \qquad \dfrac{v_1 \times v_2 : (\tau_{\text{Light}}, d)}{v_1 : (\tau_{\text{Light}}, d)}\ \textsc{Conv-Reflect}}{\exists a_1 : d \times \mathsf{channel\_count}(\tau_{\text{Light}}) \mid v_1 = \tau_{\text{Light}}(a_1)}\ \textsc{Conv-BasicInit}$$

$$\dfrac{v_2 \in v_B \qquad \dfrac{v_1 \times v_2 : (\tau_{\text{Light}}, d)}{v_2 : (\tau_{\text{Reflectance}}, d)}\ \textsc{Conv-Reflect}}{\exists a_2 : d \times \mathsf{channel\_count}(\tau_{\text{Reflectance}}) \mid v_2 = \tau_{\text{Reflectance}}(a_2)}\ \textsc{Conv-BasicInit}$$

$$\dfrac{\dfrac{}{\tau_{\text{Light}}(a_1) \times \tau_{\text{Reflectance}}(a_2) \to \tau_{\text{Light}}((a_1) \times (a_2))}\ \textsc{E-Reflect} \qquad \exists a_1 : d \times \mathsf{channel\_count}(\tau_{\text{Light}}) \mid v_1 = \tau_{\text{Light}}(a_1)}{\exists a_1 : d \times \mathsf{channel\_count}(\tau_{\text{Light}}) \mid v_1 \times \tau_{\text{Reflectance}}(a_2) \to \tau_{\text{Light}}((a_1) + (a_2))}\ \textsc{Subst}$$

$$\dfrac{\exists a_1 : d \times \mathsf{channel\_count}(\tau_{\text{Light}}) \mid v_1 \times \tau_{\text{Reflectance}}(a_2) \to \tau_{\text{Light}}((a_1) \times (a_2)) \qquad \exists a_2 : d \times \mathsf{channel\_count}(\tau_{\text{Reflectance}}) \mid v_2 = \tau_{\text{Light}}(a_2)}{\exists a_1 : d \times \mathsf{channel\_count}(\tau_{\text{Light}}), a_2 : d \times \mathsf{channel\_count}(\tau_{\text{Reflectance}}) \mid v_1 \times v_2 \to \tau_{\text{Light}}((a_1) \times (a_2))}\ \textsc{Subst}$$

Since $v_1 \times v_2 \to \tau_{\text{Light}}((a_1) \times (a_2))$, progress holds for this case.

**Summary.** Since the progress theorem holds for both cases of the LightAdd rule, the LightAdd rule satisfies the progress theorem. Any non-basic value that is type checked by the LightAdd rule can be further evaluated.

### 4.3.6 Progress Summary

We have shown that each SmallerSpace type rule fulfills the progress theorem by the principle of induction. Therefore, any type checked SmallerSpace non-basic value can be evaluated further. SmallerSpace satisfies the progress theorem.

## 4.4 Preservation Theorem

**Theorem.** A non-basic typed value $v$ can be evaluated to $v'$ according to the progress theorem. $v : (\tau, d)$ implies $v' : (\tau, d)$. The theorem is more formally stated below:

$$\frac{v : (\tau, d) \qquad v \rightarrow v'}{v' : (\tau, d)} \text{ PRESERVATION}$$

We will utilize structural induction to prove the preservation theorem. The inductive hypothesis is as follows:

$$\frac{v_i \subset v \qquad v_i : (\tau_i, d_i) \qquad v_i \rightarrow v_i'}{v_i' : (\tau_i, d_i)} \text{ PRES-INDHYP}$$

### 4.4.1 Init Preservation

$$\frac{\alpha : d \times \mathsf{channel\_count}(\tau)}{\tau(\alpha) : (\tau, d)} \text{ INIT}$$

**Case 1:** $\alpha \in \mathbb{A}$**.** If $\alpha$ is an array literal, $\tau(\alpha)$ is a basic value and cannot be evaluated further. Therefore, the preservation theorem holds for this case.

**Case 2:** $\alpha \notin \mathbb{A}$**.**

$$\frac{\dfrac{\dfrac{\alpha \notin \mathbb{A}}{\exists \alpha' \mid \alpha \rightarrow \alpha'} \text{ ARRAY-PROGRESS} \qquad \dfrac{\tau(\alpha) : (\tau, d)}{\alpha : d \times \mathsf{channel\_count}(\tau)} \text{ CONV-INIT}}{\exists \alpha' : d \times \mathsf{channel\_count}(\tau) \mid \alpha \rightarrow \alpha'} \text{ ARRAY-PRESERVATION}}{\exists \alpha' : d \times \mathsf{channel\_count}(\tau) \mid \tau(\alpha) \rightarrow \tau(\alpha')} \text{ E-PROPINIT}$$

$$\frac{\alpha' : d \times \mathsf{channel\_count}(\tau)}{\tau(\alpha') : (\tau, d)} \text{ INIT}$$

Since $\tau(\alpha) : (\tau, d)$, $\tau(\alpha) \rightarrow \tau(\alpha')$, and $\tau(\alpha') : (\tau, d)$, preservation holds for this case.

**Summary.** Preservation holds for both cases of the INIT rule. Any non-basic type that INIT type checks can be evaluated further (PROGRESS). The type of the non-basic value is preserved after the evaluation step.

### 4.4.2 Cast Preservation

$$\frac{v : (\tau_1, d) \qquad \mathsf{path\_exists}(\tau_1, \tau_2)}{\tau_2(v) : (\tau_2, d)} \text{ CAST}$$

**Case 1:** $v \notin v_B$ If $v \notin v_B$, we know that there exists some $v'$ such that $\tau_2(v) \rightarrow \tau_2(v')$ by the progress theorem. By the inductive hypothesis, $v$ has the same type as $v'$.

$$\frac{v : (\tau_1, d) \qquad \mathsf{path\_exists}(\tau_1, \tau_2)}{\tau_2(v) : (\tau_2, d)} \text{ CAST}$$

$$\frac{v' : (\tau_1, d) \qquad \mathsf{path\_exists}(\tau_1, \tau_2)}{\tau_2(v') : (\tau_2, d)} \text{ CAST}$$

Since $\tau_2(v) : (\tau_2, d)$, $\tau_2(v) \rightarrow \tau_2(v')$, and $\tau_2(v') : (\tau_2, d)$, preservation holds for this case.

**case 2:** $v \in v_B$**,** $\tau_1 = \tau_2$**.**

$$\dfrac{\dfrac{v \in v_B \qquad \dfrac{\tau_2(v) : (\tau_2, d)}{\exists \tau_1 \mid v : (\tau_1, d)}\textsc{Conv-Cast}}{\exists \tau_1, a_1 : d \times \mathsf{channel\_count}(\tau_1) \mid v = \tau_1(a_1)}\textsc{Conv-BasicInit} \qquad \dfrac{\tau_1 = \tau_2 \qquad \dfrac{}{\tau_1(\tau_1(a_1)) \to \tau_1(a_1)}\textsc{E-CastTrivial}}{\tau_2(\tau_1(a_1)) \to \tau_2(a_1)}\textsc{Subst}}{\exists \tau_1, a_1 : d \times \mathsf{channel\_count}(\tau_1) \mid \tau_2(v) \to \tau_2(a_1)}\textsc{Subst}$$

$$\dfrac{\dfrac{a_1 : d \times \mathsf{channel\_count}(\tau_1) \qquad \tau_1 = \tau_2}{a_1 : d \times \mathsf{channel\_count}(\tau_2)}\textsc{Subst}}{\tau_2(a_1) : (\tau_2, d)}\textsc{Init}$$

Since $\tau_2(v) : (\tau_2, d)$, $\tau_2(v) \to \tau_2(a_1)$, and $\tau_2(a_1) : (\tau_2, d)$, preservation holds for this case.

**Case 3:** $v \in v_B$**,** $\tau_1$ **adjacent to** $\tau_2$**.** We know that there exists a corresponding adjacent casting rule for $\tau_1$ and $\tau_2$. We will show that preservation holds for $\tau_1 = \tau_{\text{Light}}$ and $\tau_2 = \tau_{\text{LMS}}$. Other proofs for this case are similar in form.

$$\dfrac{\dfrac{v \in v_B \qquad \dfrac{\tau_1 = \tau_{\text{Light}} \qquad \dfrac{\tau_2(v) : (\tau_2, d)}{\exists \tau_1 \mid v : (\tau_1, d)}\textsc{Conv-Cast}}{v : (\tau_{\text{Light}}, d)}\textsc{Subst}}{\exists a : d \times \mathsf{channel\_count}(\tau_{\text{Light}}) \mid v = \tau_{\text{Light}}(a)}\textsc{Conv-BasicInit} \qquad \dfrac{\tau_2 = \tau_{\text{LMS}} \qquad \dfrac{}{\tau_{\text{LMS}}(\tau_{\text{Light}}(a)) \to \tau_{\text{LMS}}(\mathsf{matmul}(a, M_{\textsc{Light2LMS}}))}\textsc{E-Light2LMS}}{\tau_2(\tau_{\text{Light}}(a)) \to \tau_{\text{LMS}}(\mathsf{matmul}(a, M_{\textsc{Light2LMS}}))}\textsc{Subst}}{\tau_2(v) \to \tau_{\text{LMS}}(\mathsf{matmul}(a, M_{\textsc{Light2LMS}}))}\textsc{Subst}$$

$$\dfrac{\tau_2 = \tau_{\text{LMS}} \qquad \dfrac{\dfrac{\mathsf{channel\_count}(\tau_{\text{LMS}}) = 3 \qquad \dfrac{M_{\textsc{Light2LMS}} : 89 \times 3 \qquad \dfrac{a : d \times \mathsf{channel\_count}(\tau_{\text{Light}}) \qquad \mathsf{channel\_count}(\tau_{\text{Light}}) = 89}{a : d \times 89}\textsc{Subst}}{\mathsf{matmul}(a, M_{\textsc{Light2LMS}}) : d \times 3}\textsc{E-ArrMatMul}}{\mathsf{matmul}(a, M_{\textsc{Light2LMS}}) : d \times \mathsf{channel\_count}(\tau_{\text{LMS}})}\textsc{Subst}}{\tau_{\text{LMS}}(\mathsf{matmul}(a, M_{\textsc{Light2LMS}})) : (\tau_{\text{LMS}}, d)}\textsc{Init}}{\tau_{\text{LMS}}(\mathsf{matmul}(a, M_{\textsc{Light2LMS}})) : (\tau_2, d)}\textsc{Subst}$$

Since $\tau_2(v) : (\tau_2, d)$, $\tau_2(v) \to \tau_{\text{LMS}}(\mathsf{matmul}(a, M_{\textsc{Light2LMS}}))$, and $\tau_{\text{LMS}}(\mathsf{matmul}(a, M_{\textsc{Light2LMS}})) : (\tau_2, d)$, preservation holds for this sub-case. Other sub-cases (i.e., $\tau_1 = \tau_{\text{XYZ}}$ and $\tau_2 = \tau_{\text{LMS}}$) come to the same conclusion.

**Case 4:** $v \in v_B$**,** $\tau_1$ **not adjacent to** $\tau_2$**.** Like case 4 of the Cast progress proof, we will demonstrate this case for when $\tau_1 = \tau_{\text{Light}}$ and $\tau_2 = \tau_{\text{XYZ}}$. The proof for other pairs of types are similar in form.

$$\dfrac{\tau_2 = \tau_{\text{XYZ}} \qquad \dfrac{\mathsf{path\_exists}(\tau_{\text{Light}}, \tau_{\text{XYZ}}) \qquad 1 \leq \mathsf{distance}(\tau_{\text{LMS}}, \tau_{\text{XYZ}}) \leq \mathsf{distance}(\tau_{\text{Light}}, \tau_{\text{XYZ}}) \qquad \mathsf{distance}(\tau_{\text{Light}}, \tau_{\text{LMS}}) = 1}{\tau_{\text{XYZ}}(\tau_{\text{Light}}(a)) \to \tau_{\text{XYZ}}(\tau_{\text{LMS}}(\tau_{\text{Light}}(a)))}\textsc{E-CastHop}}{\tau_2(\tau_{\text{Light}}(a)) \to \tau_2(\tau_{\text{LMS}}(\tau_{\text{Light}}(a)))}\textsc{Subst}$$

$$\dfrac{\tau_2(\tau_{\text{Light}}(a)) \to \tau_2(\tau_{\text{LMS}}(\tau_{\text{Light}}(a))) \qquad \dfrac{v \in v_B \qquad \dfrac{\tau_1 = \tau_{\text{Light}} \qquad \dfrac{\tau_2(v) : (\tau_2, d)}{\exists \tau_1 \mid v : (\tau_1, d)}\textsc{Conv-Cast}}{v : (\tau_{\text{Light}}, d)}\textsc{Subst}}{\exists a \times \mathsf{channel\_count}(\tau_{\text{Light}}) \mid v = \tau_{\text{Light}}(a)}\textsc{Conv-BasicInit}}{\tau_2(v) \to \tau_2(\tau_{\text{LMS}}(v))}\textsc{Subst}$$

$$\dfrac{\dfrac{v : (\tau_1, d) \qquad \dfrac{\tau_1 = \tau_{\text{Light}} \qquad \mathsf{path\_exists}(\tau_{\text{Light}}, \tau_{\text{LMS}})}{\mathsf{path\_exists}(\tau_1, \tau_{\text{LMS}})}\textsc{Subst}}{\tau_{\text{LMS}}(v) : (\tau_{\text{LMS}}, d)}\textsc{Cast} \qquad \dfrac{\tau_2 = \tau_{\text{XYZ}} \qquad \mathsf{path\_exists}(\tau_{\text{LMS}}, \tau_{\text{XYZ}})}{\mathsf{path\_exists}(\tau_{\text{LMS}}, \tau_2)}\textsc{Subst}}{\tau_2(\tau_{\text{LMS}}(v)) : (\tau_2, d)}\textsc{Cast}$$

Since $\tau_2(v) : (\tau_2, d)$, $\tau_2(v) \to \tau_2(\tau_{\text{LMS}}(v))$, and $\tau_2(\tau_{\text{LMS}}(v)) : (\tau_2, d)$, preservation holds for this sub-case. Other sub-cases (i.e., $\tau_1 = \tau_{\text{LMS}}$ and $\tau_2 = \tau_{\text{sRGB}}$) come to the same conclusion.

**Summary.** Preservation holds for all cases of the Cast rule. Any non-basic type that Cast type checks can be evaluated further (Progress). The type of the non-basic value is preserved after the evaluation step.

### 4.4.3 TristimulusAdd Preservation

$$\frac{v_1, v_2 : (\tau_{\text{tristimulus}}, d)}{v_1 + v_2 : (\tau_{\text{tristimulus}}, d)} \text{ TristimulusAdd}$$

**Case 1: $v_1 \notin v_B$ and/or $v_2 \notin v_B$.** We know from case 1 of the TristimulusAdd progress proof that there exists some $v_1'$ or $v_2'$ such that $v_1 + v_2 \to v_1' + v_2$ or $v_1 + v_2 \to v_1 + v_2'$. By the inductive hypothesis we can conclude that $v_1'$ and $v_2'$ have the same shaped types as $v_1$ and $v_2$. Therefore, by the TristimulusAdd rule, $v_1 + v_2$ is the same type as $v_1' + v_2$ or $v_1 + v_2'$. Thus, preservation holds for case 1.

**Case 2: $v_1, v_2 \in v_B$.** We can see from the Conv-TristimulusAdd rule that both $v_1$ and $v_2$ must share the same shaped type. A different evaluation rule may apply to the value depending on what tristimulus type $v_1$ and $v_2$ share. We will exhaustively cover every possible tristimulus type case.

**Case 2-a:** $v_1, v_2 : (\tau_{\mathbf{XYZ}}, d)$ We know from case 2-a of the progress proof for TristimulusAdd that $\exists a_1, a_2 : d \times \mathsf{channel\_count}(\tau_{\text{XYZ}}) \mid v_1 + v_2 \to \tau_{\text{XYZ}}((a_1) + (a_2))$.

$$\cfrac{a_1, a_2 : d \times \mathsf{channel\_count}(\tau_{\text{XYZ}}) \qquad \cfrac{}{\mathsf{broadcastable}(d \times \mathsf{channel\_count}(\tau_{\text{XYZ}}), d \times \mathsf{channel\_count}(\tau_{\text{XYZ}}))} \text{ TrivialBroadcast}}{\cfrac{(a_1) + (a_2) : d \times \mathsf{channel\_count}(\tau_{\text{XYZ}})}{\tau_{\text{XYZ}}((a_1) + (a_2)) : (\tau_{\text{XYZ}}, d)} \text{ Init}} \text{ ArrayBinOpR}$$

Since $v_1 + v_2 : (\tau_{\text{XYZ}}, d)$, $v_1 + v_2 \to \tau_{\text{XYZ}}((a_1) + (a_2))$, and $\tau_{\text{XYZ}}((a_1) + (a_2)) : (\tau_{\text{XYZ}}, d)$, preservation holds for this case.

**Case 2-b:** $v_1, v_2 : (\tau_{\mathbf{LMS}}, d)$ We know from case 2-b of the progress proof for TristimulusAdd that $\exists a_1, a_2 : d \times \mathsf{channel\_count}(\tau_{\text{LMS}}) \mid v_1 + v_2 \to \tau_{\text{LMS}}((a_1) + (a_2))$.

$$\cfrac{a_1, a_2 : d \times \mathsf{channel\_count}(\tau_{\text{LMS}}) \qquad \cfrac{}{\mathsf{broadcastable}(d \times \mathsf{channel\_count}(\tau_{\text{LMS}}), d \times \mathsf{channel\_count}(\tau_{\text{LMS}}))} \text{ TrivialBroadcast}}{\cfrac{(a_1) + (a_2) : d \times \mathsf{channel\_count}(\tau_{\text{LMS}})}{\tau_{\text{LMS}}((a_1) + (a_2)) : (\tau_{\text{LMS}}, d)} \text{ Init}} \text{ ArrayBinOpR}$$

Since $v_1 + v_2 : (\tau_{\text{LMS}}, d)$, $v_1 + v_2 \to \tau_{\text{LMS}}((a_1) + (a_2))$, and $\tau_{\text{LMS}}((a_1) + (a_2)) : (\tau_{\text{LMS}}, d)$, preservation holds for this case.

**Case 3-b:** $v_1, v_2 : (\tau_{\mathbf{sRGB}}, d)$ We know from case 2-c of the progress proof for TristimulusAdd that $\exists a_1, a_2 : d \times \mathsf{channel\_count}(\tau_{\text{sRGB}}) \mid v_1 + v_2 \to \tau_{\text{sRGB}}((((((a_1)/([255]))**(\gamma_{\tau_{\text{sRGB}}})) + (((a_2)/([255]))**((\gamma_{\tau_{\text{sRGB}}})))) * *(\gamma^{-1}_{\tau_{\text{sRGB}}})) \times ([255]))$.

In order to show that $\tau_{\text{sRGB}}((((((a_1)/([255]))**(\gamma_{\tau_{\text{sRGB}}})) + (((a_2)/([255]))**((\gamma_{\tau_{\text{sRGB}}}))))**(\gamma^{-1}_{\tau_{\text{sRGB}}})) \times ([255])) : (\tau_{\text{sRGB}}, d)$, we must show that $(((((a_1)/([255]))**(\gamma_{\tau_{\text{sRGB}}})) + (((a_2)/([255]))**((\gamma_{\tau_{\text{sRGB}}}))))**(\gamma^{-1}_{\tau_{\text{sRGB}}})) \times ([255]) : d \times \mathsf{channel\_count}(\tau_{\text{sRGB}})$.

All operations in the above array expression are binary array operations, and can be evaluated by the rules E-ArrBinOpL and E-ArrBinOpR. These rules stipulate that the left operand must be broadcastable to the right operand, or vice versa. $a_1$ and $a_2$ both have the same dimension, $d \times \mathsf{channel\_count}(\tau_{\text{sRGB}})$. [255], $\gamma_{\tau_{\text{sRGB}}}$, $\gamma^{-1}_{\tau_{\text{sRGB}}}$ all have the dimension of 1, and thus can be broadcast to $d \times \mathsf{channel\_count}(\tau_{\text{sRGB}})$ by the ScalarBroadcast rule.

The output of the rules E-ArrBinOpL and E-ArrBinOpR has the dimension type of the dimension being broadcast to. (In $\mathsf{broadcastable}(d_1, d_2)$, $d_1$ is being broadcast to $d_2$.) Therefore, the final dimension type of $(((((a_1)/([255])) * *(\gamma_{\tau_{\text{sRGB}}})) + (((a_2)/([255])) * *((\gamma_{\tau_{\text{sRGB}}})))) * *(\gamma^{-1}_{\tau_{\text{sRGB}}})) \times ([255])$ is $d \times \mathsf{channel\_count}(\tau_{\text{sRGB}})$.

$$\frac{(((((a_1)/([255])) * *(\gamma_{\tau_{\text{sRGB}}})) + (((a_2)/([255])) * *((\gamma_{\tau_{\text{sRGB}}})))) * *(\gamma^{-1}_{\tau_{\text{sRGB}}})) \times ([255]) : d \times \mathsf{channel\_count}(\tau_{\text{sRGB}})}{\tau_{\text{sRGB}}((((((a_1)/([255])) * *(\gamma_{\tau_{\text{sRGB}}})) + (((a_2)/([255])) * *((\gamma_{\tau_{\text{sRGB}}})))) * *(\gamma^{-1}_{\tau_{\text{sRGB}}})) \times ([255])) : (\tau_{\text{sRGB}}, d)} \text{ Init}$$

Since $v_1 + v_2 : (\tau_{\text{sRGB}}, d)$, $v_1 + v_2 \to \tau_{\text{sRGB}}((((((a_1)/([255])) * *(\gamma_{\tau_{\text{sRGB}}})) + (((a_2)/([255])) * *((\gamma_{\tau_{\text{sRGB}}})))) * *(\gamma^{-1}_{\tau_{\text{sRGB}}})) \times ([255]))$, and $\tau_{\text{sRGB}}((((((a_1)/([255]))**(\gamma_{\tau_{\text{sRGB}}})) + (((a_2)/([255]))**((\gamma_{\tau_{\text{sRGB}}}))))**(\gamma^{-1}_{\tau_{\text{sRGB}}})) \times ([255])) : (\tau_{\text{sRGB}}, d)$, preservation holds for this case.

**Summary.** Preservation holds for all cases of the TristimulusAdd rule. Any non-basic type that TristimulusAdd type checks can be evaluated further (Progress). The type of the non-basic value is preserved after the evaluation step.

### 4.4.4 LightAdd Preservation

$$\dfrac{v_1, v_2 : (\tau_{\text{Light}}, d)}{v_1 + v_2 : (\tau_{\text{Light}}, d)}\ \textsc{LightAdd}$$

**Case 1:** $v_1 \notin v_B$**.** Since $v_1$ is not in $v_B$, we know from the progress theorem that there exists some $v_1'$ such that $v_1 \to v_1'$. Additionally, from the preservation inductive hypothesis, we know that $v_1'$ is of the same type as $v_1$.

$$\dfrac{\dfrac{v_1 \notin v_B}{\exists v_1' \mid v_1 \to v_1'}\ \textsc{Progress}}{\exists v_1' \mid v_1 + v_2 \to v_1' + v_2}\ \textsc{E-PropBinOpL}$$

$$\dfrac{\dfrac{\dfrac{v_1 + v_2 : (\tau_{\text{Light}}, d)}{v_1 : (\tau_{\text{Light}}, d)}\ \textsc{Conv-LightAdd} \qquad v_1 \to v_1'}{v_1' : (\tau_{\text{Light}}, d)}\ \textsc{Pres-IndHyp} \qquad \dfrac{v_1 + v_2 : (\tau_{\text{Light}}, d)}{v_2 : (\tau_{\text{Light}}, d)}\ \textsc{Conv-LightAdd}}{v_1' + v_2 : (\tau_{\text{Light}}, d)}\ \textsc{LightAdd}$$

Since $v_1 + v_2 : (\tau_{\text{Light}}, d)$, $v_1 + v_2 \to v_1' + v_2$, and $v_1' + v_2 : (\tau_{\text{Light}}, d)$, preservation holds for this case.

**Case 2:** $v_2 \notin v_B$**.** Since $v_2$ is not in $v_B$, we know from the progress theorem that there exists some $v_2'$ such that $v_2 \to v_2'$. Additionally, from the preservation inductive hypothesis, we know that $v_2'$ is of the same type as $v_2$.

$$\dfrac{\dfrac{v_2 \notin v_B}{\exists v_2' \mid v_2 \to v_2'}\ \textsc{Progress}}{\exists v_2' \mid v_1 + v_2 \to v_1 + v_2'}\ \textsc{E-PropBinOpR}$$

$$\dfrac{\dfrac{\dfrac{v_1 + v_2 : (\tau_{\text{Light}}, d)}{v_2 : (\tau_{\text{Light}}, d)}\ \textsc{Conv-LightAdd} \qquad v_2 \to v_2'}{v_2' : (\tau_{\text{Light}}, d)}\ \textsc{Pres-IndHyp} \qquad \dfrac{v_1 + v_2 : (\tau_{\text{Light}}, d)}{v_1 : (\tau_{\text{Light}}, d)}\ \textsc{Conv-LightAdd}}{v_1 + v_2' : (\tau_{\text{Light}}, d)}\ \textsc{LightAdd}$$

Since $v_1 + v_2 : (\tau_{\text{Light}}, d)$, $v_1 + v_2 \to v_1 + v_2'$, and $v_1 + v_2' : (\tau_{\text{Light}}, d)$, preservation holds for this case.

**Case 3:** $v_1, v_2 \notin v_B$**.** For this case, the proofs from both case 1 and case 2 apply. Therefore, preservation holds for this case.

**Case 4:** $v_1, v_2 \in v_B$**.** Case 2 of the progress proof for the LightAdd rule has the same stipulations as this case. We know from case 2 of the progress proof that $\exists a_1, a_2 : d \times \mathsf{channel\_count}(\tau_{\text{Light}}) \mid v_1 + v_2 \to \tau_{\text{Light}}((a_1) + (a_2))$.

$$\dfrac{\dfrac{a_1, a_2 : d \times \mathsf{channel\_count}(\tau_{\text{Light}}) \qquad \dfrac{}{\mathsf{broadcastable}(d \times \mathsf{channel\_count}(\tau_{\text{Light}}), d \times \mathsf{channel\_count}(\tau_{\text{Light}}))}\ \textsc{TrivialBroadcast}}{(a_1) + (a_2) : d \times \mathsf{channel\_count}(\tau_{\text{Light}})}\ \textsc{ArrayBinOpR}}{\tau_{\text{Light}}((a_1) + (a_2)) : (\tau_{\text{Light}}, d)}\ \textsc{Init}$$

Since $v_1 + v_2 : (\tau_{\text{Light}}, d)$, $v_1 + v_2 \to \tau_{\text{Light}}((a_1) + (a_2))$, and $\tau_{\text{Light}}((a_1) + (a_2)) : (\tau_{\text{Light}}, d)$, preservation holds for this case.

**Summary.** Preservation holds for all cases of the LightAdd rule. Any non-basic type that LightAdd type checks can be evaluated further (Progress). The type of the non-basic value is preserved after the evaluation step.

### 4.4.5 Reflect Preservation

$$\dfrac{v_1 : (\tau_{\text{Light}}, d) \qquad v_2 : (\tau_{\text{Reflectance}}, d)}{v_1 \times v_2 : (\tau_{\text{Light}}, d)}\ \textsc{Reflect}$$

**Case 1:** $v_1 \notin v_B$**.** Since $v_1$ is not in $v_B$, we know from the progress theorem that there exists some $v_1'$ such that $v_1 \to v_1'$. Additionally, from the preservation inductive hypothesis, we know that $v_1'$ is of the same type as $v_1$.

$$\dfrac{\dfrac{v_1 \notin v_B}{\exists v_1' \mid v_1 \to v_1'}\ \textsc{Progress}}{\exists v_1' \mid v_1 \times v_2 \to v_1' \times v_2}\ \textsc{E-PropBinOpL}$$

$$\dfrac{\dfrac{\dfrac{v_1 \times v_2 : (\tau_{\text{Light}}, d)}{v_1 : (\tau_{\text{Light}}, d)}\ \textsc{Conv-Reflect} \qquad v_1 \to v_1'}{v_1' : (\tau_{\text{Light}}, d)}\ \textsc{Pres-IndHyp} \qquad \dfrac{v_1 \times v_2 : (\tau_{\text{Light}}, d)}{v_2 : (\tau_{\text{Reflectance}}, d)}\ \textsc{Conv-Reflect}}{v_1' \times v_2 : (\tau_{\text{Light}}, d)}\ \textsc{Reflect}$$

Since $v_1 \times v_2 : (\tau_{\text{Light}}, d)$, $v_1 \times v_2 \to v_1' \times v_2$, and $v_1' \times v_2 : (\tau_{\text{Light}}, d)$, preservation holds for this case.

**Case 2:** $v_2 \notin v_B$**.** Since $v_2$ is not in $v_B$, we know from the progress theorem that there exists some $v_2'$ such that $v_2 \to v_2'$. Additionally, from the preservation inductive hypothesis, we know that $v_2'$ is of the same type as $v_2$.

$$\dfrac{\dfrac{v_2 \notin v_B}{\exists v_2' \mid v_2 \to v_2'}\ \textsc{Progress}}{\exists v_2' \mid v_1 \times v_2 \to v_1 \times v_2'}\ \textsc{E-PropBinOpR}$$

$$\dfrac{\dfrac{\dfrac{v_1 \times v_2 : (\tau_{\text{Light}}, d)}{v_2 : (\tau_{\text{Reflectance}}, d)}\ \textsc{Conv-Reflect} \qquad v_2 \to v_2'}{v_2' : (\tau_{\text{Reflectance}}, d)}\ \textsc{Pres-IndHyp} \qquad \dfrac{v_1 \times v_2 : (\tau_{\text{Light}}, d)}{v_1 : (\tau_{\text{Light}}, d)}\ \textsc{Conv-Reflect}}{v_1 \times v_2' : (\tau_{\text{Light}}, d)}\ \textsc{Reflect}$$

Since $v_1 \times v_2 : (\tau_{\text{Light}}, d)$, $v_1 \times v_2 \to v_1 \times v_2'$, and $v_1 \times v_2' : (\tau_{\text{Light}}, d)$, preservation holds for this case.

**Case 3:** $v_1, v_2 \notin v_B$**.** For this case, the proofs from both case 1 and case 2 apply. Therefore, preservation holds for this case.

**Case 4:** $v_1, v_2 \in v_B$**.** We know from case 3 of the progress proof that $\exists a_1 : d \times \mathsf{channel\_count}(\tau_{\text{Light}}), a_2 : d \times \mathsf{channel\_count}(\tau_{\text{Reflectance}}) \mid v_1 \times v_2 \to \tau_{\text{Light}}((a_1) \times (a_2))$.

$$\dfrac{\dfrac{\mathsf{channel\_count}(\tau_{\text{Light}}) = 89 \qquad \mathsf{channel\_count}(\tau_{\text{Reflectance}}) = 89}{\mathsf{channel\_count}(\tau_{\text{Light}}) = \mathsf{channel\_count}(\tau_{\text{Reflectance}})}\ \textsc{Subst} \qquad a_2 : d \times \mathsf{channel\_count}(\tau_{\text{Reflectance}})}{a_2 : d \times \mathsf{channel\_count}(\tau_{\text{Light}})}\ \textsc{Subst}$$

$$\dfrac{\dfrac{a_1, a_2 : d \times \mathsf{channel\_count}(\tau_{\text{Light}}) \qquad \dfrac{}{\mathsf{broadcastable}(d \times \mathsf{channel\_count}(\tau_{\text{Light}}), d \times \mathsf{channel\_count}(\tau_{\text{Light}}))}\ \textsc{TrivialBroadcast}}{(a_1) \times (a_2) : d \times \mathsf{channel\_count}(\tau_{\text{Light}})}\ \textsc{E-ArrBinOpR}}{\tau_{\text{Light}}((a_1) \times (a_2)) : (\tau_{\text{Light}}, d)}\ \textsc{Init}$$

Since $v_1 \times v_2 : (\tau_{\text{Light}}, d)$, $v_1 \times v_2 \to \tau_{\text{Light}}((a_1) \times (a_2))$, and $\tau_{\text{Light}}((a_1) \times (a_2)) : (\tau_{\text{Light}}, d)$, preservation holds for this case.

**Summary.** Preservation holds for all cases of the Reflect rule. Any non-basic type that Reflect type checks can be evaluated further (Progress). The type of the non-basic value is preserved after the evaluation step.

### 4.4.6 Preservation Summary

We have shown that each SmallerSpace type rule fulfills the preservation theorem by the principle of induction. Any type checked SmallerSpace value that can take an evaluation step preserves its type after said evaluation step.

# 5 Equality Saturation Rewrite Rules

Tbl. 7 is a list of the rewrite rules used in our equality saturation optimizer. Part of the rules are adapted from TASO [8], which investigates rewrite rules for tensor algebra containing up to four operators. We have pruned rewrite rules that cause a substantial increase in equality saturation runtime. Rules involving the exponentiation operator (Pow) are newly introduced by us.

| | |
|---|---|
| add-associative | (Add x (Add y z)) ↔ (Add (Add x y) z) |
| add-commutative | (Add x y) ↔ (Add y x) |
| mul-associative | (Mul x (Mul y z)) ↔ (Mul (Mul x y) z) |
| mul-commutative | (Mul x y) ↔ (Mul y x) |
| matmul-is-associative | (MatMul x (MatMul y z)) ↔ (MatMul (MatMul x y) z) |
| mul-distributes-over-add | (Mul (Add x y) z) ↔ (Add (Mul x z) (Mul y z)) |
| matmul-is-linear-over-add | (MatMul x (Add y z)) ↔ (Add (MatMul x y) (MatMul x z)) |
| pow-distributes-over-mul | (Pow (Mul x y) z) ↔ (Mul (Pow x z) (Pow y z)) |
| div-distributes-over-add | (Div (Add x y) z) ↔ (Add (Div x z) (Div y z)) |

Table 7: Rewrite Rules

# 6 Benchmarking Programs in CoolerSpace

## 6.1 SpaceConv

The **SpaceConv** program converts an input image from sRGB space to opRGB space. CoolerSpace performs type checking on the conversion operation (line 13) to ensure that the conversion between the input object's type and the destination type is valid (rule Cast from Fig. 2). CoolerSpace also abstracts away the complexity of applying and removing gamma from sRGB and opRGB. This allows programmers to focus on the semantics of manipulating an image's color space without worrying about the implementation of color space conversion.

```
1  import coolerspace as cs
2  import sys
3
4  # Compilation Arguments
5  path = sys.argv[1]
6  shape_y = int(sys.argv[2])
7  shape_x = int(sys.argv[3])
8
9  # Inputs
10 srgb = cs.create_input("image", [shape_y, shape_x], cs.sRGB)
11
12 # Conversion from sRGB to opRGB
13 op = cs.opRGB(srgb)
14
15 # Compilation
16 cs.create_output(op)
17 cs.compile(path)
```

## 6.2 ColorBlindness

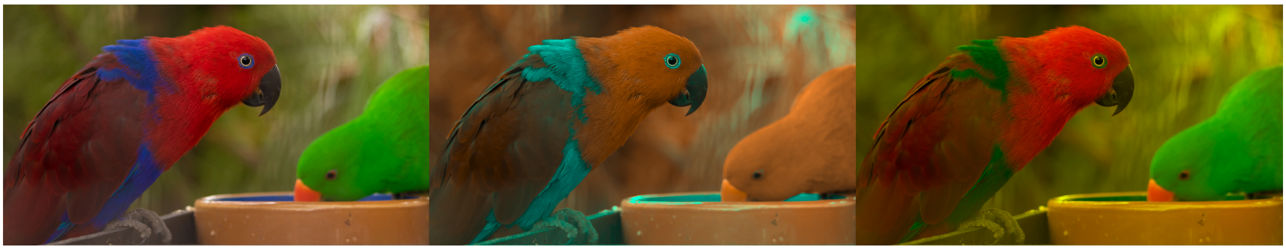


Figure 8: Color blindness simulation. Original image courtesy of Simon Amarasingham [5].

The **ColorBlindness** program takes as input an image in sRGB space and a projection matrix representing a specific type of dichromatic color blindness, and outputs an image simulating the effects of color blindness. The simulation algorithm is based on the the single-plane approach described by Viénot et al. [14].

Fig. 8 shows the output of the program for simulating Deuteranopia (a particular kind of "red-green blindness" due to the missing of M cones on the retina), and Tritanopia (missing S cones and thus cannot correctly perceive blue hues). As expected, red and green shades appear almost identical in the simulated Deuteranopia image; the simulated Tritanopia image correctly shows that Tritanopes cannot correctly perceive blue hues.

While most images are originally encoded in the sRGB space, principled color blindness simulation must be done in the LMS space. CoolerSpace automatically handles the implementation logic of casting from sRGB to LMS and back. The program also demonstrates CoolerSpace's ability to treat colors as geometric objects and to cast them using a linear transformation matrix (Line 17). This transformation is type checked to ensure that the dimensions of the image in LMS space and the colorblindness matrix are compatible for a matrix multiplication. This type checking is performed by the TriMatMul rule in Fig. 2.

```
1  import coolerspace as cs
2  import sys
3
4  # Compilation Arguments
5  path = sys.argv[1]
6  shape_y = int(sys.argv[2])
7  shape_x = int(sys.argv[3])
8
9  # Inputs
10 image = cs.create_input("image", [shape_y, shape_x], cs.sRGB)
11 colorblind_matrix = cs.create_input("colorblind_matrix", [3, 3], cs.Matrix)
```

```
# Convert image to LMS
image_lms = cs.LMS(image)

# Apply colorblindness matrix
colorblind_image_lms = cs.matmul(image_lms, colorblind_matrix)

# Convert back
colorblind_image = cs.sRGB(colorblind_image_lms)

# Compilation
cs.create_output(colorblind_image)
cs.compile(path)
```

## 6.3 Adaptation

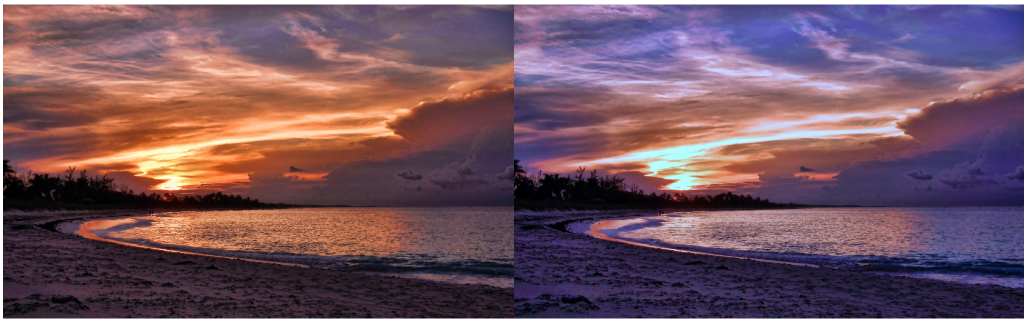


Figure 9: Chromatic adaptation simulation. Original image courtesy of Trish Hartman [7].

**Adaptation** is a program that simulates how the visual system adapts to the illuminant of a scene and preserves constant color perception across different illuminants [13]. Chromatic adaptation is the basis of white balancing in the camera raw processing pipeline [12]. The output of the program is shown in Fig. 9, where the original image captured under the CIE Standard Illuminant D35 (estimated) is adapted to one captured under the CIE Standard Illuminant D65 (typical daylight).

For principled chromatic adaptation, one must know the light spectra of the original and adapting illuminants, which are expressed in the `Light` type (Lines 10–11). CoolerSpace facilitates color space conversion between `Light`, `LMS`, and `sRGB`. Like **ColorBlindness**, it also checks to ensure that the matrix multiplication operation on the `LMS` object in line 37 is well-formed.

```
1  import coolerspace as cs
2  import sys
3
4  # Compilation Arguments
5  path = sys.argv[1]
6  shape_y = int(sys.argv[2])
7  shape_x = int(sys.argv[3])
8
9  # Inputs
10 original_illuminant = cs.create_input("original_illuminant", [1], cs.LightSpectrum)
11 target_illuminant = cs.create_input("target_illuminant", [1], cs.LightSpectrum)
12 image = cs.create_input("image", [shape_y, shape_x], cs.sRGB)
13
14 # Convert image to LMS
15 image_lms = cs.LMS(image)
16
17 # Calculating factor to adjust lms cones by
18 original_illuminant_matrix = cs.Matrix(cs.LMS(original_illuminant))
19 target_illuminant_matrix = cs.Matrix(cs.LMS(target_illuminant))
20 abc = target_illuminant_matrix / original_illuminant_matrix
21
22 # Project to diagonal matrix
23 identity_3x3 = cs.Matrix([
24     [1, 0, 0],
25     [0, 1, 0],
26     [0, 0, 1]
27 ])
28 project_to_3x3 = cs.Matrix([
```

```
    [1],
    [1],
    [1]
])
abc_3x3 = cs.matmul(project_to_3x3, abc)
abc_diagonal = abc_3x3 * identity_3x3

# Apply modulation
modulated_image_lms = cs.matmul(image_lms, abc_diagonal)
modulated_image_srgb = cs.sRGB(modulated_image_lms)

# Compilation
cs.create_output(modulated_image_srgb)
cs.compile(path)
```

### 6.4 Interpolation

**Interpolation** simulates the interpolation of two `sRGB` images. The programmer specifies on line 14 that they want to evenly interpolate the colors of the two images. Programmers often attempt to interpolate color values directly in `sRGB` space [2, 1, 4, 3], which is physically incorrect, as `sRGB` is a non-linear color space. `sRGB` channels do not scale linearly with light intensity. CoolerSpace understands that the programmer intends to mix two images evenly on line 14. CoolerSpace performs the even interpolation in linear RGB space instead of `sRGB` space, thereby avoiding a potential bug.

```
1  import coolerspace as cs
2  import sys
3
4  # Compilation arguments
5  path = sys.argv[1]
6  shape_y = int(sys.argv[2])
7  shape_x = int(sys.argv[3])
8
9  # Inputs
10 image1 = cs.create_input("image1", [shape_y, shape_x], cs.sRGB)
11 image2 = cs.create_input("image2", [shape_y, shape_x], cs.sRGB)
12
13 # Interpolate between the two images by half
14 mixed = image1 * 0.5 + image2 * 0.5
15
16 # Compilation
17 cs.create_output(mixed)
18 cs.compile(path)
```

### 6.5 Mixing

The pigment mixing implementation in CoolerSpace uses the Kubelka-Munk model to simulate the mixture of pigments. The Kubelka-Munk model [10, 9] relates the reflectance spectrum $R(\lambda)$ of a pigment to its scattering and absorption spectra as seen in Equ. 1, where $K(\lambda)$ and $S(\lambda)$ represent the absorption and scattering spectra, respectively, and $C_i$ is the concentration of the $i^{th}$ constituent pigment. The scattering and absorption spectra of a homogeneous mixture of materials can be modeled by a weighted sum [6] of the spectra of the constituent pigments. This relationship is expressed in Equ. 2.

$$R(\lambda) = 1 + \frac{K(\lambda)}{S(\lambda)} - \sqrt{\frac{K(\lambda)^2}{S(\lambda)^2} + 2\frac{K(\lambda)}{S(\lambda)}} \tag{1}$$

$$K_{mix}(\lambda) = \frac{1}{N}\sum_{i}^{N} K_i(\lambda) \times C_i, \quad S_{mix}(\lambda) = \frac{1}{N}\sum_{i}^{N} S_i(\lambda) \times C_i \tag{2}$$

Pigment mixing is a complex phenomenon to accurately model. CoolerSpace abstracts away the complexity of the K-M model and allows the programmer to simulate pigment mixing through a single call of the `mix(·)` function. The `mix(·)` function correctly enforces that pigment mixing be done in the spectral space. The output of the mixing, `mixed`, in line 26 is still of a `Pigment` Type. We then cast `mixed` to a `Reflectance` Type (line 29) to calculate the color of the mixture (lines 31–35) under a user-input light (line 19).

```
1  import coolerspace as cs
2  import sys
3
```

```
# Compilation Arguments
path = sys.argv[1]
shape_y = int(sys.argv[2])
shape_x = int(sys.argv[3])

# Inputs
s1 = cs.create_input("scattering1", [shape_y, shape_x], cs.ScatteringSpectrum)
s2 = cs.create_input("scattering2", [shape_y, shape_x], cs.ScatteringSpectrum)

a1 = cs.create_input("absorption1", [shape_y, shape_x], cs.AbsorptionSpectrum)
a2 = cs.create_input("absorption2", [shape_y, shape_x], cs.AbsorptionSpectrum)

d1 = cs.create_input("density1", [shape_y, shape_x, 1], cs.Matrix)
d2 = cs.create_input("density2", [shape_y, shape_x, 1], cs.Matrix)

light = cs.create_input("light", [shape_y, shape_x], cs.LightSpectrum)

# Pigment creation
p1 = cs.Pigment(s1, a1)
p2 = cs.Pigment(s2, a2)

# Mix
mixed = cs.mix(d1, p1, d2, p2)

# Cast to reflectance
reflectance = cs.ReflectanceSpectrum(mixed)

# Reflect lights off pigment reflectance
reflected = cs.LightSpectrum(cs.Matrix(light) * cs.Matrix(reflectance))

# Convert to sRGB
image = cs.sRGB(reflected)

# Compilation
cs.create_output(image)
cs.compile(path)
```

## 6.6 LAB2HSV

The process of converting to and from LAB and HSV is extremely complicated, because both are non-linear perceptual color spaces. CoolerSpace not only type checks the casting operation to ensure that an image expressed in LAB space can be converted to HSV space, but also handles the complex color space transformation logic behind the scenes. All the programmer has to do is express a single casting operation, as seen in line 13.

```
1  import coolerspace as cs
2  import sys
3
4  # Compilation Arguments
5  path = sys.argv[1]
6  shape_y = int(sys.argv[2])
7  shape_x = int(sys.argv[3])
8
9  # Inputs
10 lab = cs.create_input("image", [shape_y, shape_x], cs.LAB)
11
12 # Simple conversion
13 hsv = cs.HSV(lab)
14
15 # Compilation
16 cs.create_output(hsv)
17 cs.compile(path)
```

# References


[1] Answer to "adding/mixing colors in HSV Space". https://stackoverflow.com/a/7388476, September 2011.

[2] Answer to "Interpolate from one color to another". https://stackoverflow.com/a/21010385, January 2014.

[3] Weird interpolation between colors in hsv? https://stackoverflow.com/q/37471461, May 2016.

[4] How to calculate (a physical) ratio of colors to achieve a target color? https://math.stackexchange.com/q/4335003, December 2021.

[5] Simon Amarasingham. Red and green Eclectus Parrots, December 2019.

[6] DR Duncan. The colour of pigment mixtures. *Proceedings of the Physical Society*, 52(3):390, 1940.

[7] Trish Hartmann. Eleuthera Sunset, November 2012.

[8] Zhihao Jia, Oded Padon, James Thomas, Todd Warszawski, Matei Zaharia, and Alex Aiken. Taso: optimizing deep learning computation with automatic generation of graph substitutions. In *Proceedings of the 27th ACM Symposium on Operating Systems Principles*, pages 47–62, 2019.

[9] Paul Kubelka. New contributions to the optics of intensely light-scattering materials. part i. *Josa*, 38(5):448–457, 1948.

[10] Paul Kubelka and Franz Munk. An article on optics of paint layers. *Z. Tech. Phys*, 12(593-601):259–274, 1931.

[11] ONNX. Open neural network exchange. https://github.com/onnx/onnx, 2018.

[12] D Andrew Rowlands. Color conversion matrices in digital cameras: a tutorial. *Optical Engineering*, 59(11):110801, 2020.

[13] Andrew Stockman and David H Brainard. Color vision mechanisms. *The Optical Society of America Handbook of Optics*, 3:11–1, 2010.

[14] Françoise Viénot, Hans Brettel, and John D Mollon. Digital video colourmaps for checking the legibility of displays by dichromats. *Color Research & Application*, 24(4):243–252, 1999.

[15] Günther Wyszecki and Walter Stanley Stiles. *Color science: concepts and methods, quantitative data and formulae*, volume 40. John wiley & sons, 2000.
